# Supplementary material for: Exploiting Data Longevity for Enhancing the Lifetime of Flash-based Storage Class Memory
Source: arXiv:1704.05138 source file (2017-04-17)
Supplement: Supplementary file 1 [file appendix.tex]

%\section{APPENDIX}

\section{Sensitivity Tests: Varying Voltage Drift Distances (Weak and Strong)}

We provide the PWE analysis in the Weak and Strong devices for all other 13 workloads, which are not shown in Section \ref{sec:sense-drift}.

\begin{figure*}
\centering
	\begin{subfigure}{.33\linewidth}
		\centering
		\includegraphics[width=0.99\linewidth]{graphs-app/pwe-hm_0-weak.eps}
		\caption{hm\textunderscore0 in Weak}\label{fig:pwe-sense-drift-hm_0-weak}
	\end{subfigure}
	\begin{subfigure}{.33\linewidth}
		\centering
		\includegraphics[width=0.99\linewidth]{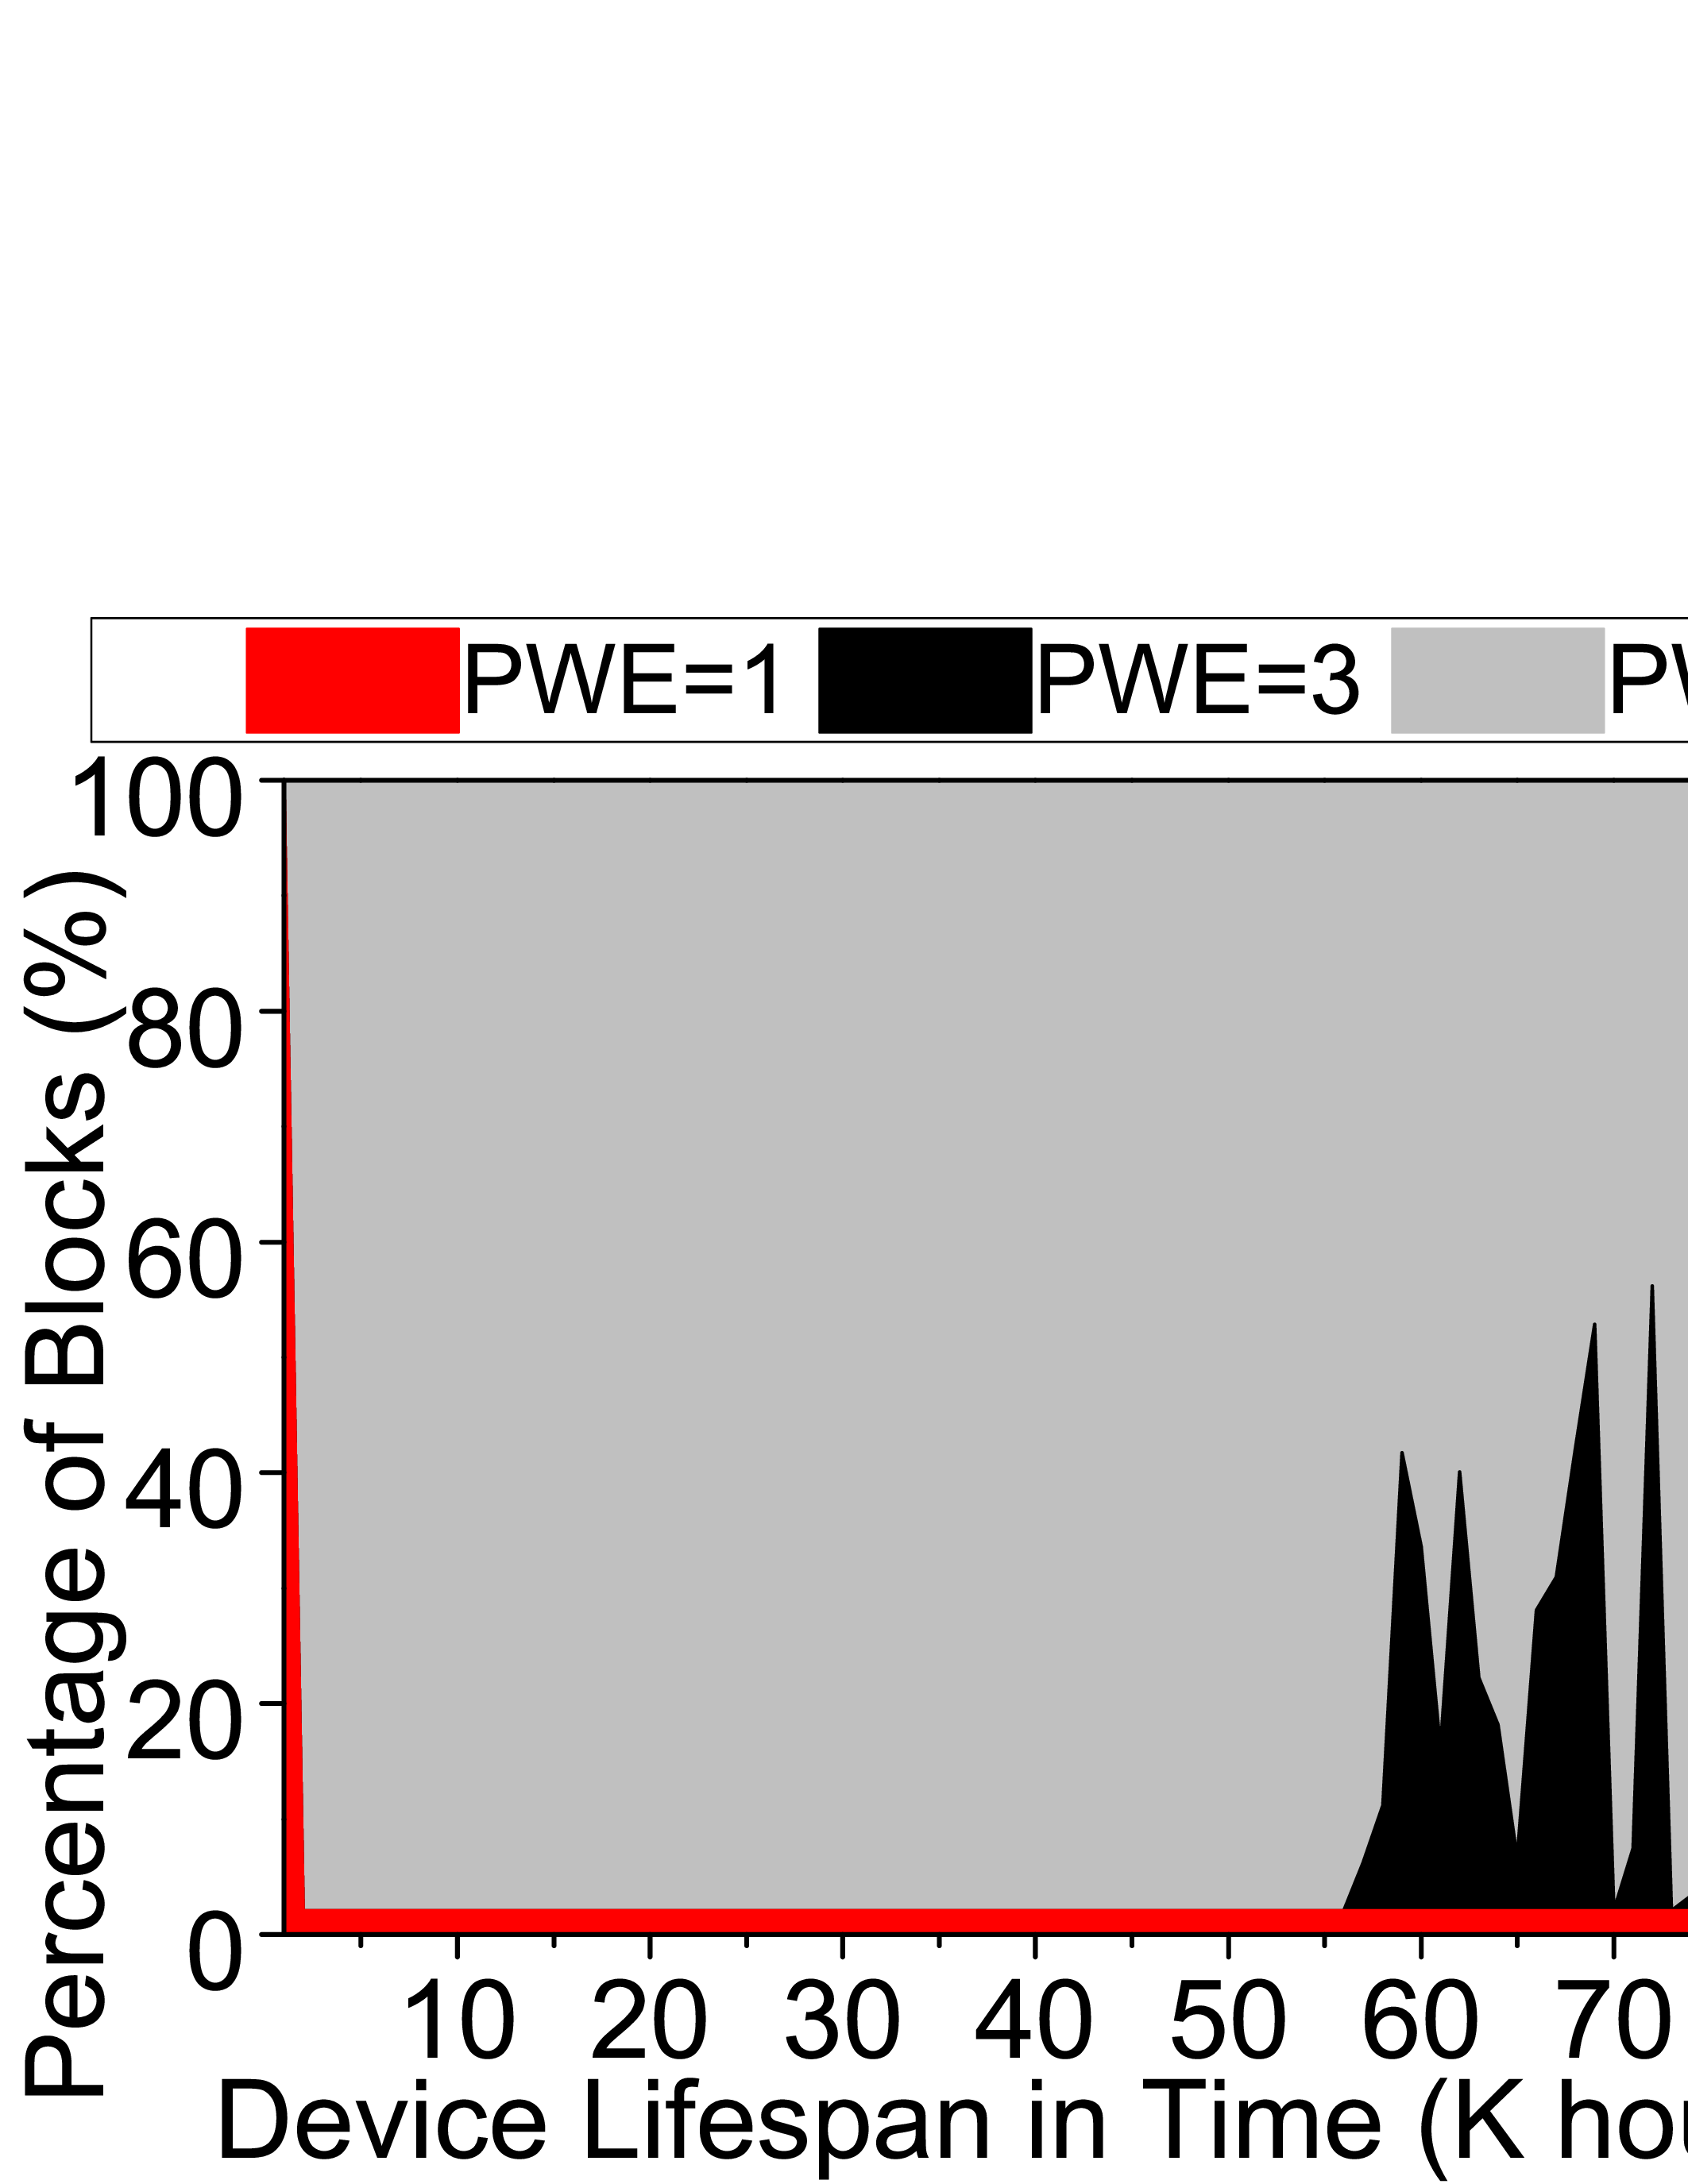}
		\caption{hm\textunderscore0 in Normal}\label{fig:pwe-sense-drift-hm_0-normal}
	\end{subfigure}
	\begin{subfigure}{.33\linewidth}
		\centering
		\includegraphics[width=0.99\linewidth]{graphs-app/pwe-hm_0-strong.eps}
		\caption{hm\textunderscore0 in Strong}\label{fig:pwe-sense-drift-hm_0-strong}
	\end{subfigure}
\caption{Percentages of blocks with 2, 4, and 8 states, when running \emph{hm\textunderscore0} on Weak, Normal, and Strong devices.}
\label{fig:pwe-sense-drift-hm_0}
\end{figure*}

\begin{figure*}
\centering
	\begin{subfigure}{.33\linewidth}
		\centering
		\includegraphics[width=0.99\linewidth]{graphs-app/pwe-prn_1-weak.eps}
		\caption{prn\textunderscore1 in Weak}\label{fig:pwe-sense-drift-prn_1-weak}
	\end{subfigure}
	\begin{subfigure}{.33\linewidth}
		\centering
		\includegraphics[width=0.99\linewidth]{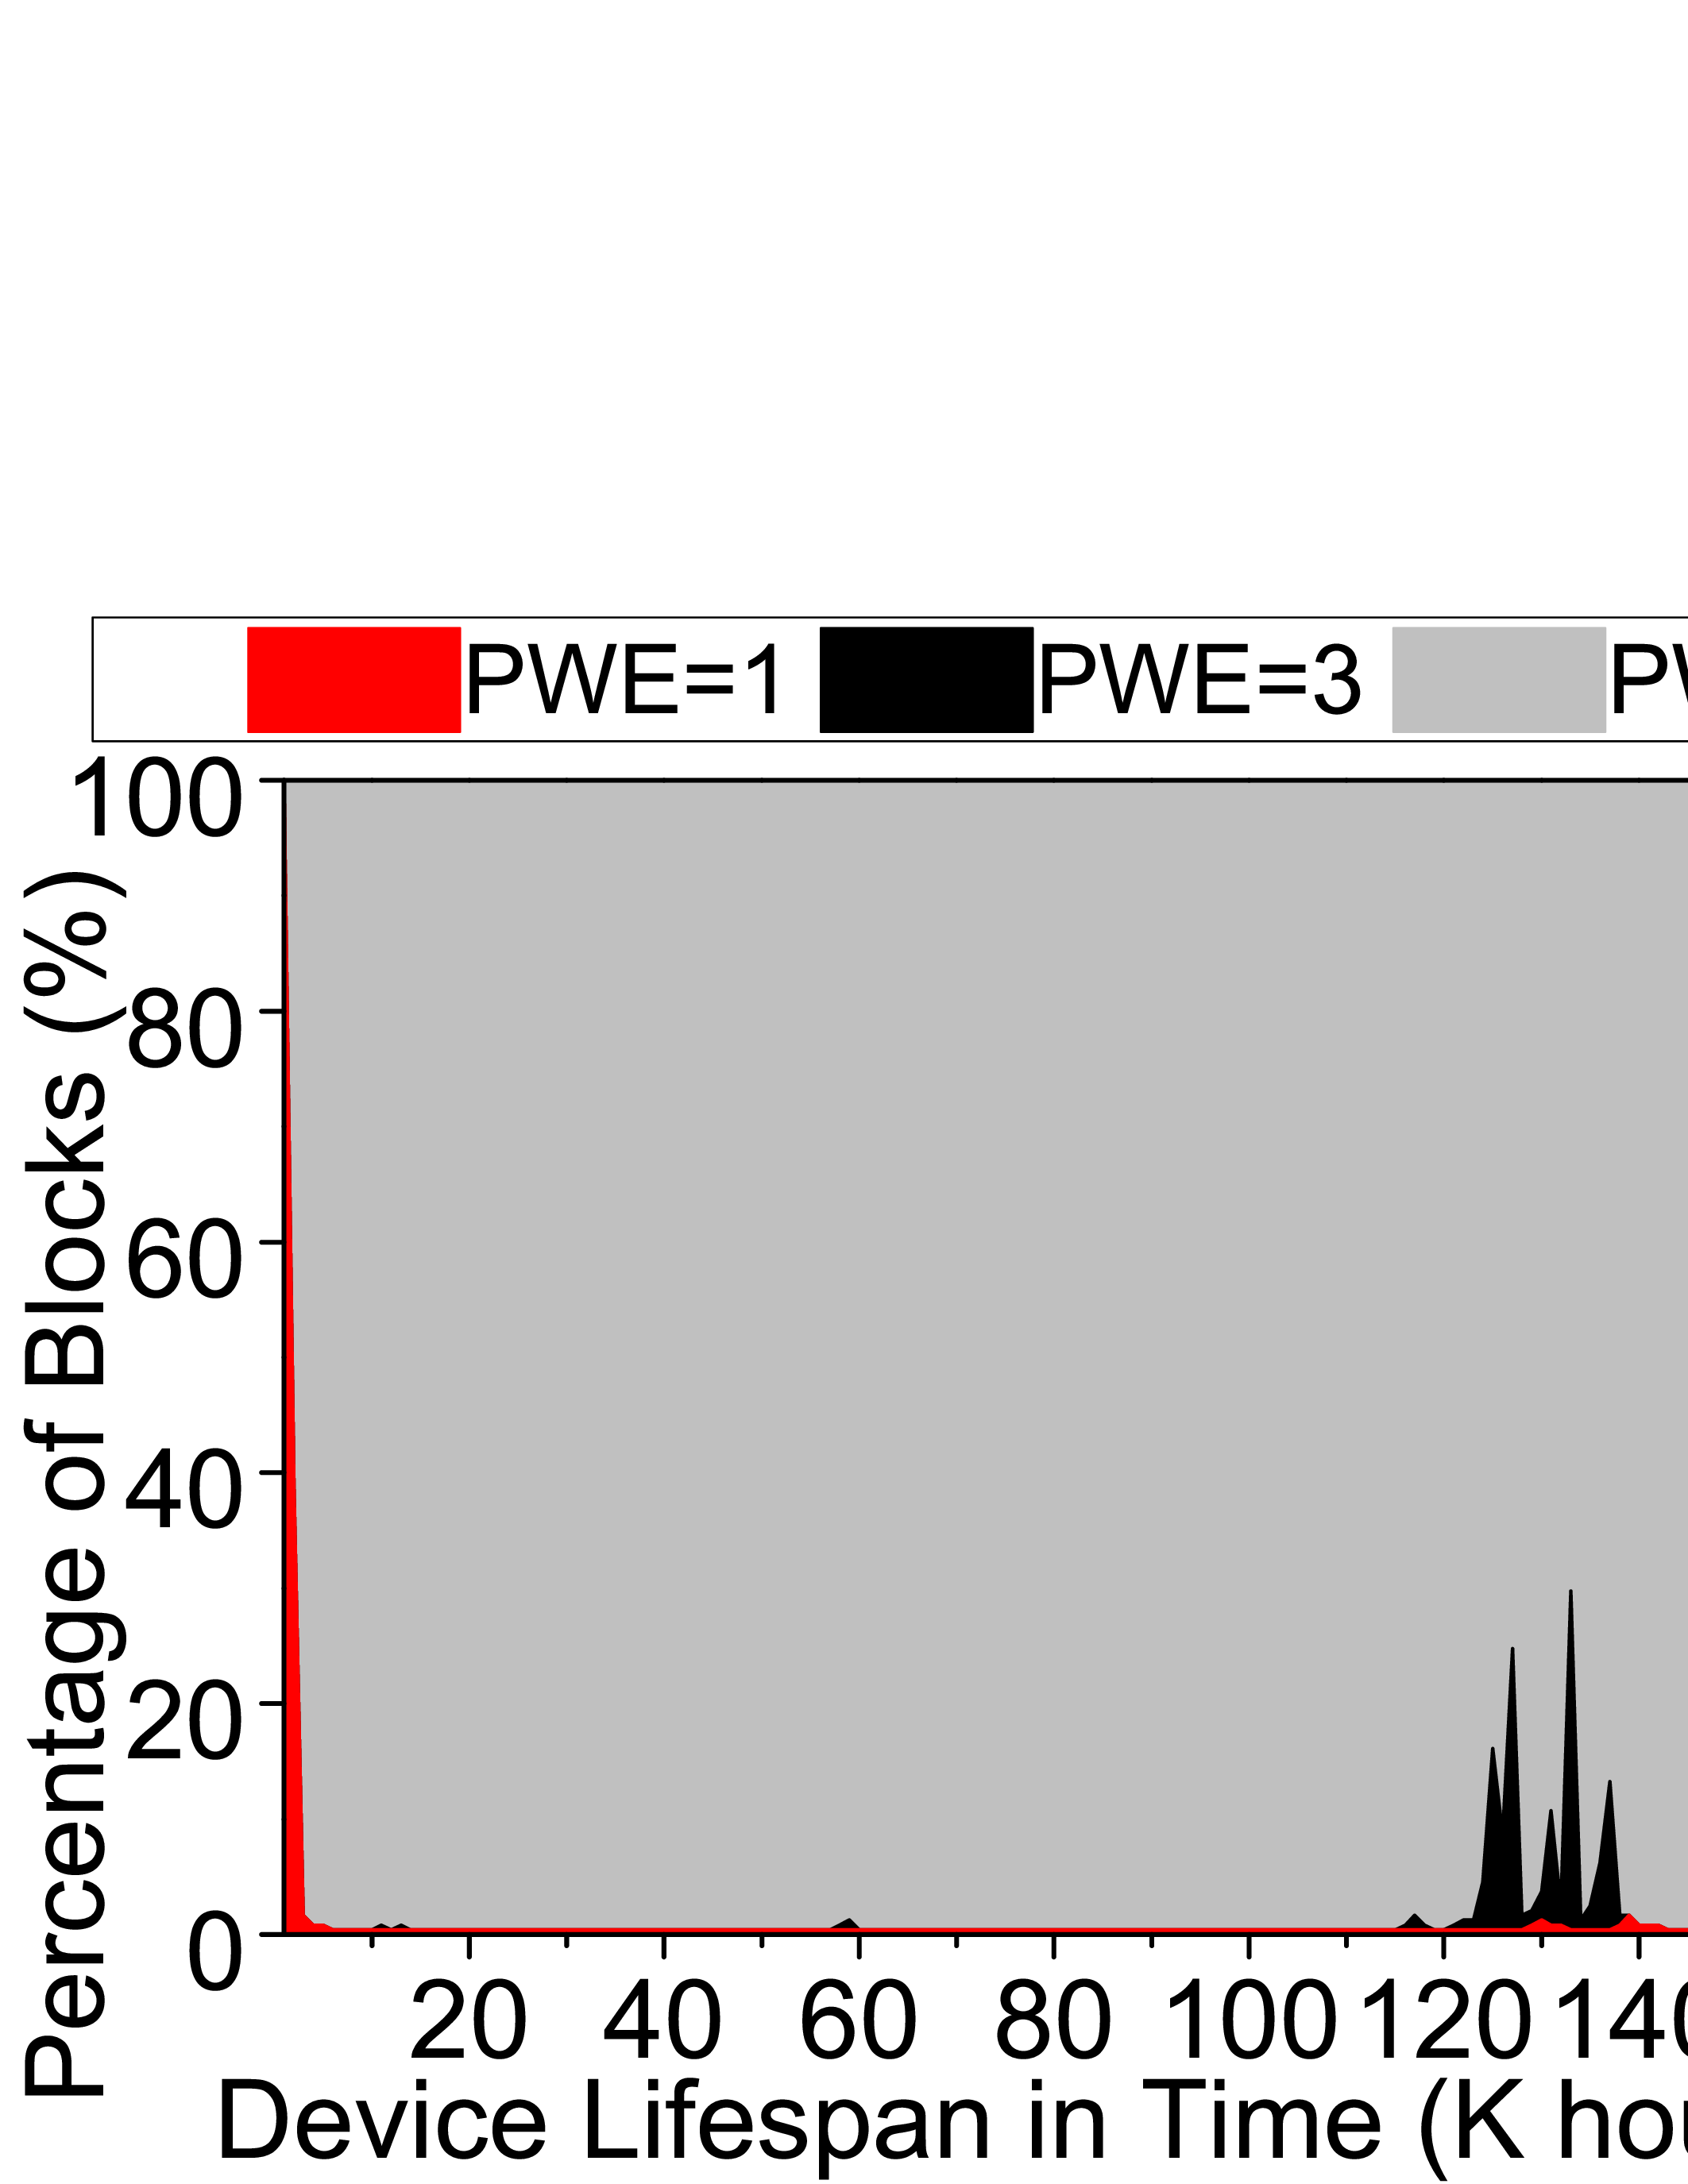}
		\caption{prn\textunderscore1 in Normal}\label{fig:pwe-sense-drift-prn_1-normal}
	\end{subfigure}
	\begin{subfigure}{.33\linewidth}
		\centering
		\includegraphics[width=0.99\linewidth]{graphs-app/pwe-prn_1-strong.eps}
		\caption{prn\textunderscore1 in Strong}\label{fig:pwe-sense-drift-prn_1-strong}
	\end{subfigure}
\caption{Percentages of blocks with 2, 4, and 8 states, when running \emph{prn\textunderscore1} on Weak, Normal, and Strong devices.}
\label{fig:pwe-sense-drift-prn_1}
\end{figure*}

\begin{figure*}
\centering
	\begin{subfigure}{.33\linewidth}
		\centering
		\includegraphics[width=0.99\linewidth]{graphs-app/pwe-proj_0-weak.eps}
		\caption{proj\textunderscore0 in Weak}\label{fig:pwe-sense-drift-proj_0-weak}
	\end{subfigure}
	\begin{subfigure}{.33\linewidth}
		\centering
		\includegraphics[width=0.99\linewidth]{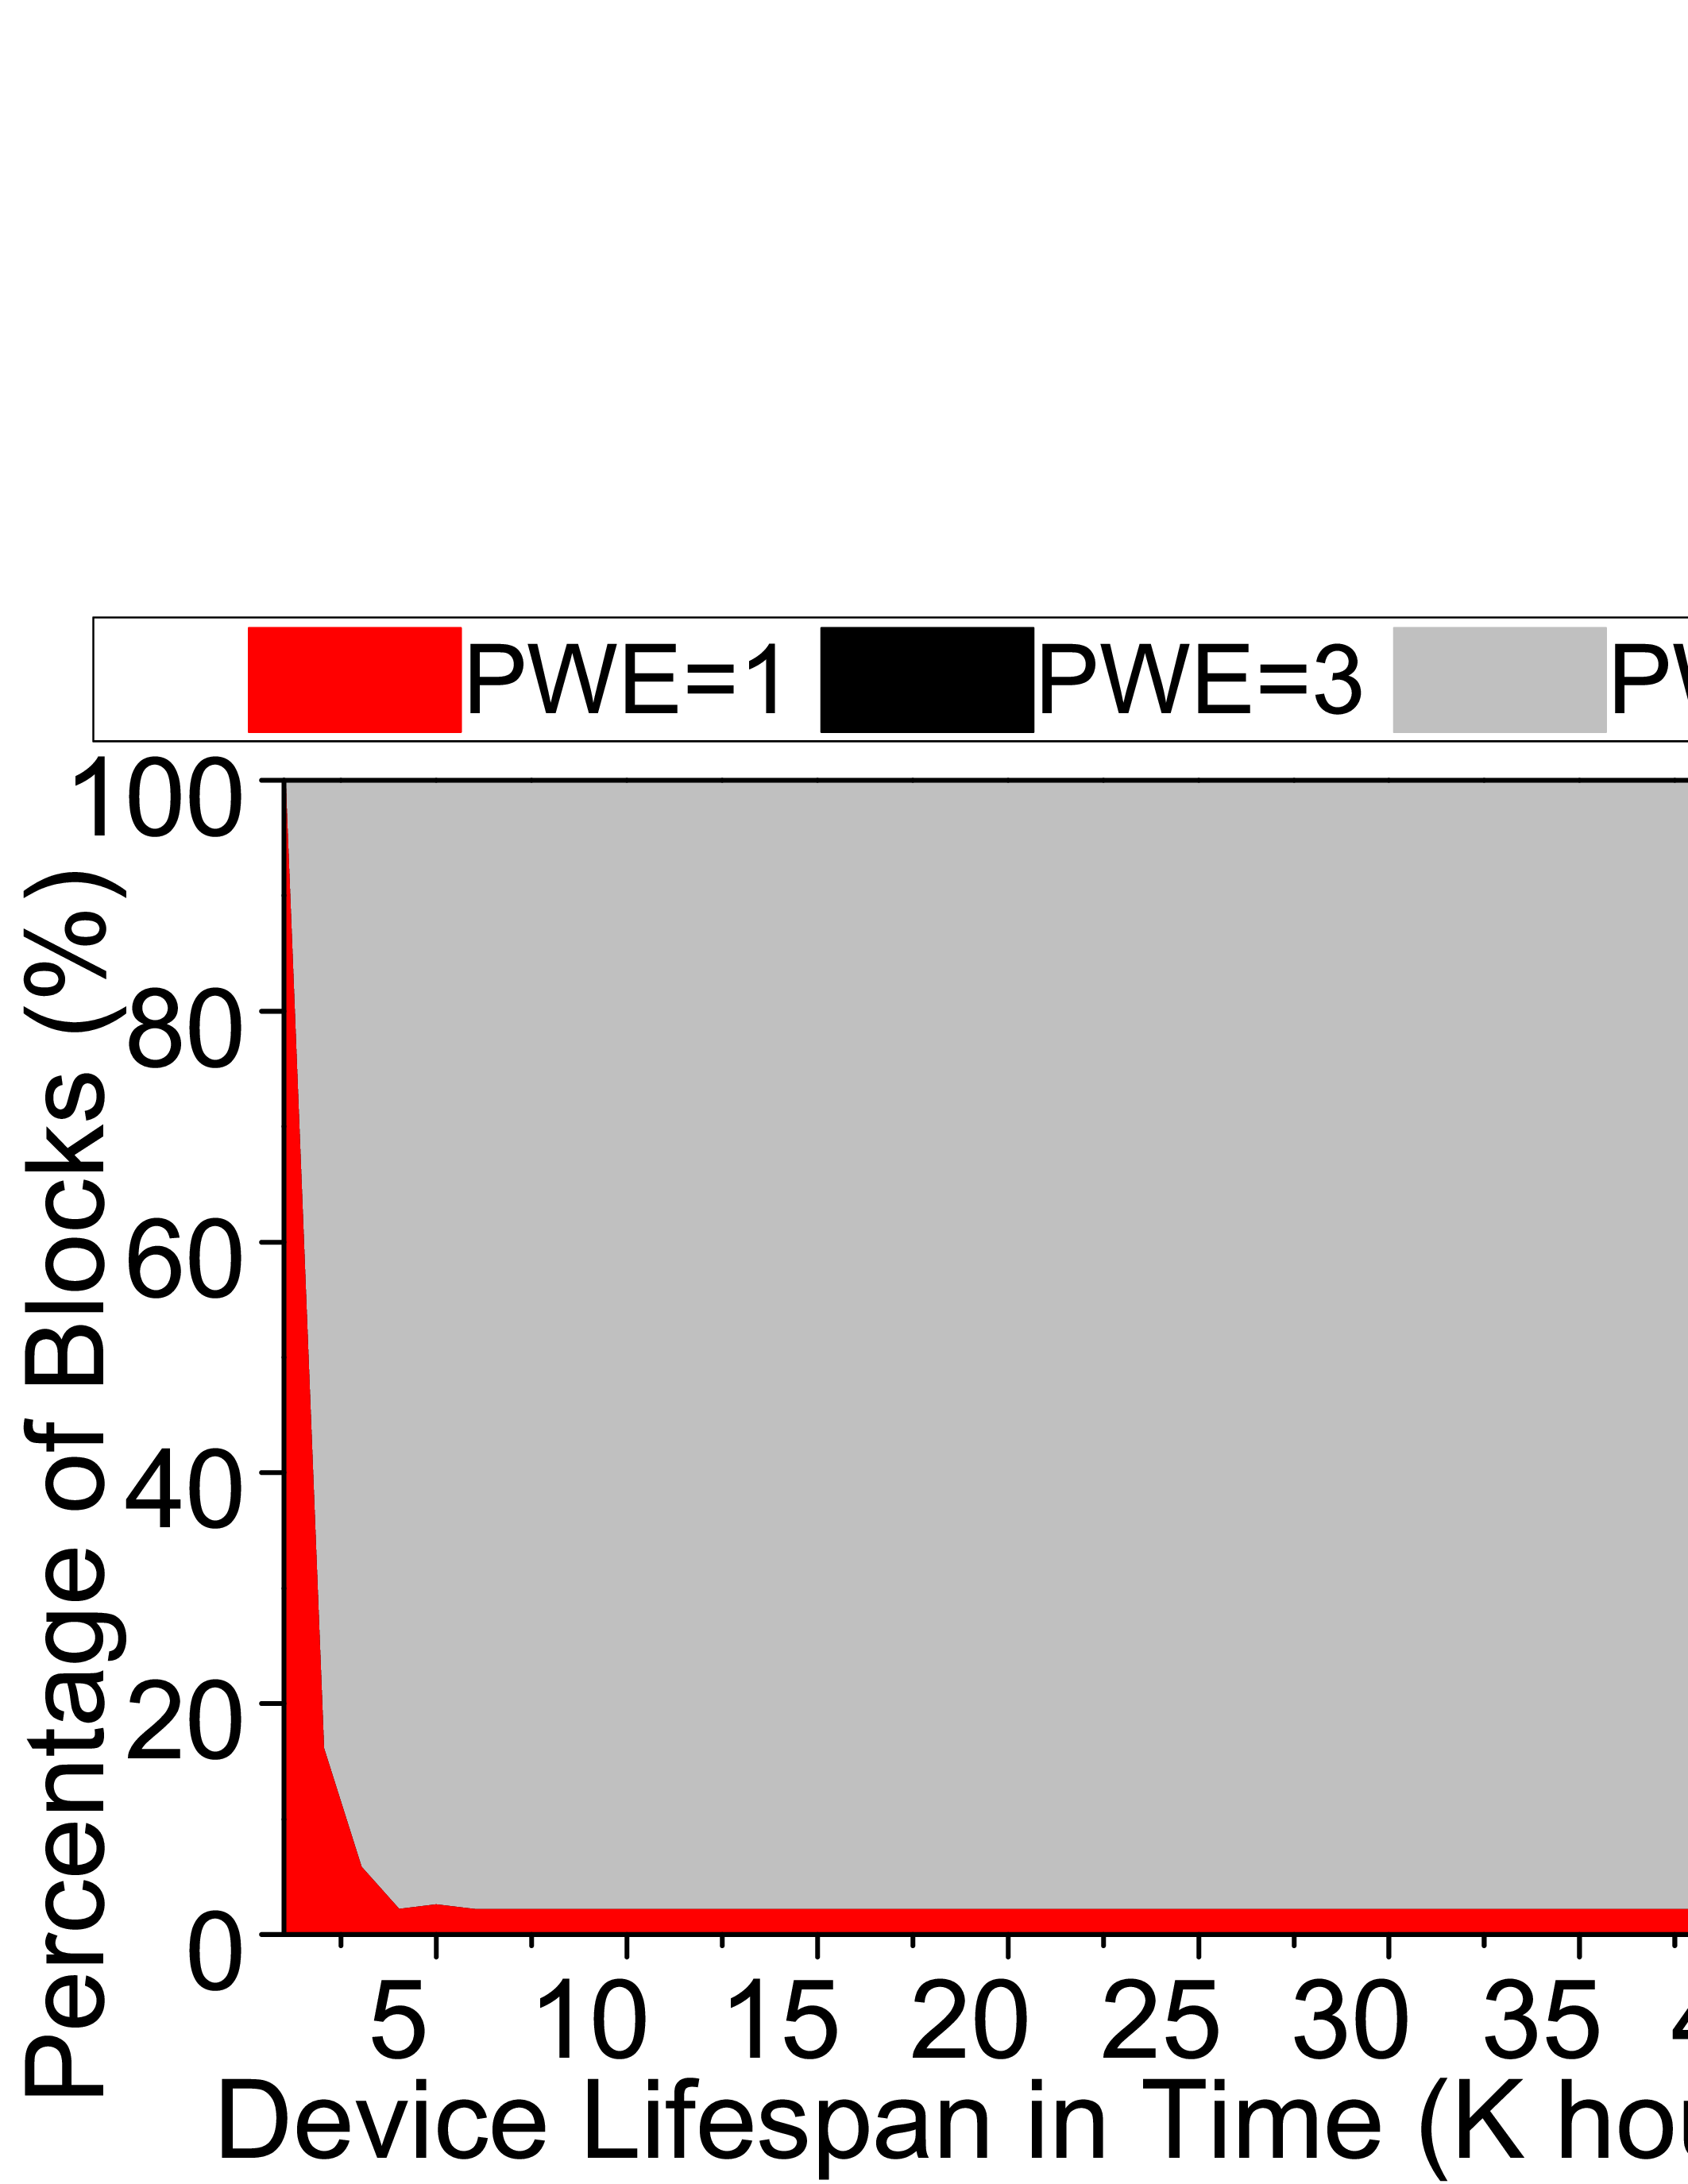}
		\caption{proj\textunderscore0 in Normal}\label{fig:pwe-sense-drift-proj_0-normal}
	\end{subfigure}
	\begin{subfigure}{.33\linewidth}
		\centering
		\includegraphics[width=0.99\linewidth]{graphs-app/pwe-proj_0-strong.eps}
		\caption{proj\textunderscore0 in Strong}\label{fig:pwe-sense-drift-proj_0-strong}
	\end{subfigure}
\caption{Percentages of blocks with 2, 4, and 8 states, when running \emph{proj\textunderscore0} on Weak, Normal, and Strong devices.}
\label{fig:pwe-sense-drift-proj_0}
\end{figure*}

\begin{figure*}
\centering
	\begin{subfigure}{.33\linewidth}
		\centering
		\includegraphics[width=0.99\linewidth]{graphs-app/pwe-prxy_0-weak.eps}
		\caption{prxy\textunderscore0 in Weak}\label{fig:pwe-sense-drift-prxy_0-weak}
	\end{subfigure}
	\begin{subfigure}{.33\linewidth}
		\centering
		\includegraphics[width=0.99\linewidth]{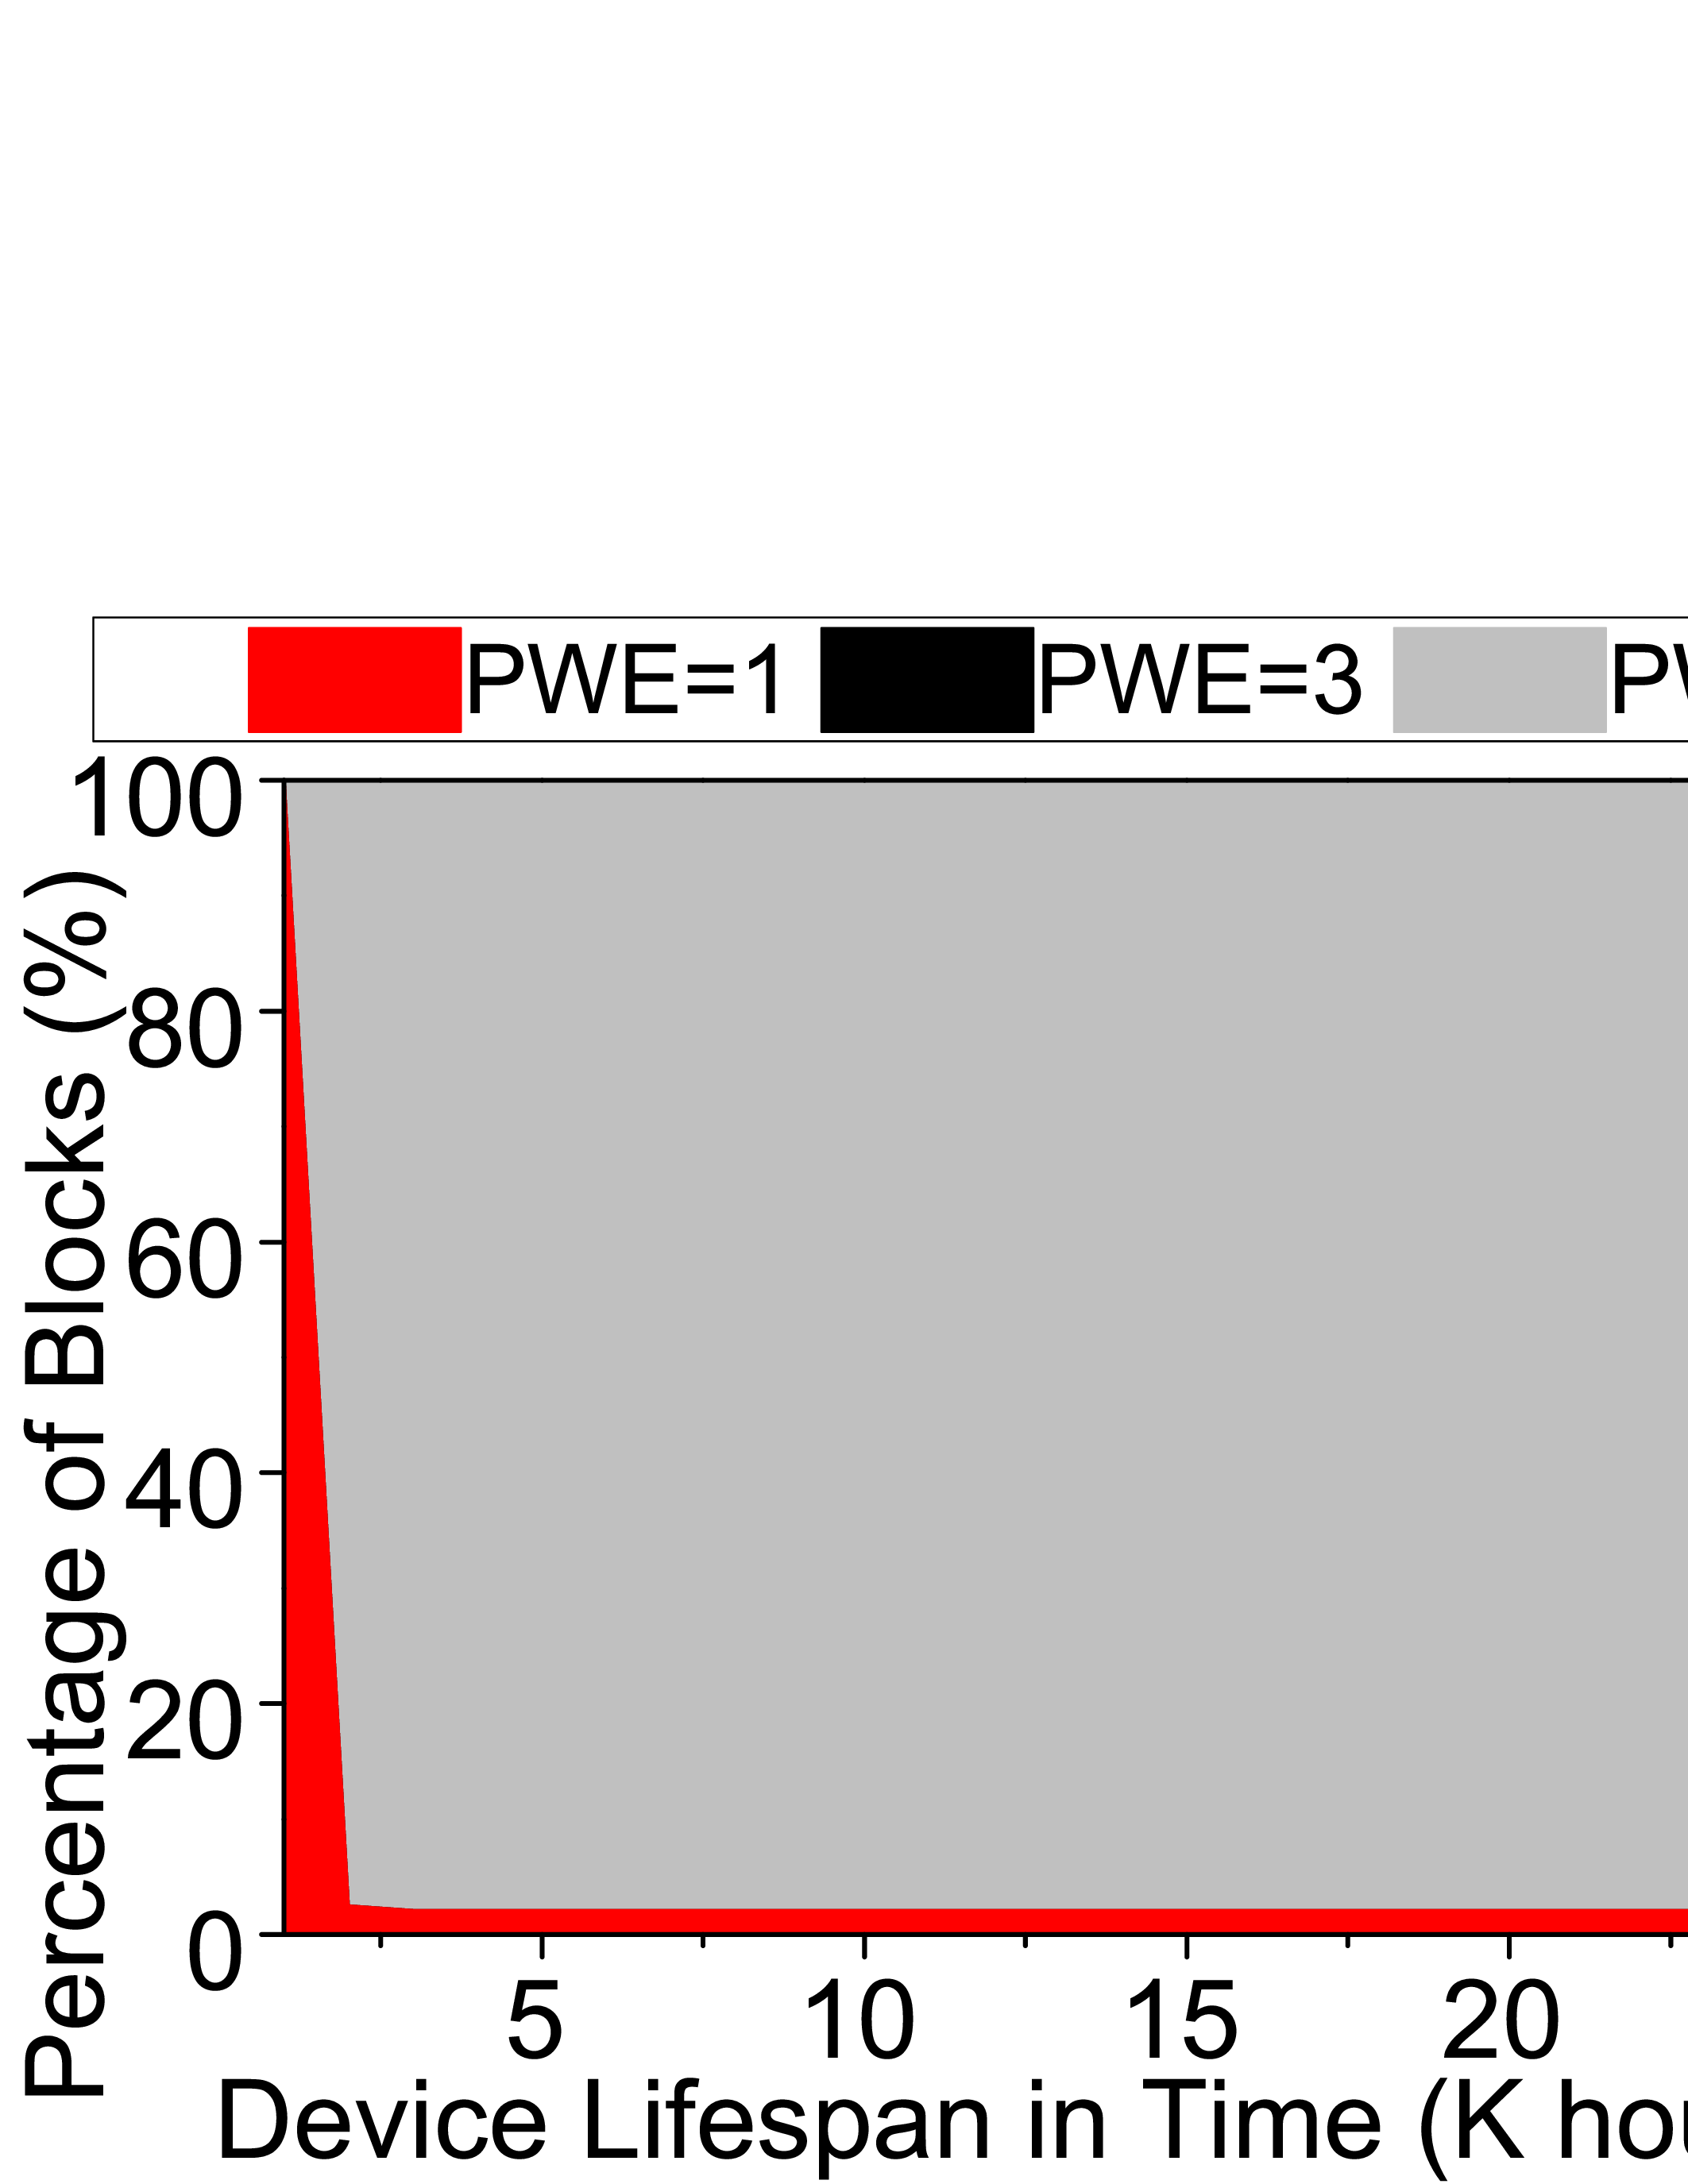}
		\caption{prxy\textunderscore0 in Normal}\label{fig:pwe-sense-drift-prxy_0-normal}
	\end{subfigure}
	\begin{subfigure}{.33\linewidth}
		\centering
		\includegraphics[width=0.99\linewidth]{graphs-app/pwe-prxy_0-strong.eps}
		\caption{prxy\textunderscore0 in Strong}\label{fig:pwe-sense-drift-prxy_0-strong}
	\end{subfigure}
\caption{Percentages of blocks with 2, 4, and 8 states, when running \emph{prxy\textunderscore0} on Weak, Normal, and Strong devices.}
\label{fig:pwe-sense-drift-prxy_0}
\end{figure*}

\begin{figure*}
\centering
	\begin{subfigure}{.33\linewidth}
		\centering
		\includegraphics[width=0.99\linewidth]{graphs-app/pwe-mds_0-weak.eps}
		\caption{mds\textunderscore0 in Weak}\label{fig:pwe-sense-drift-mds_0-weak}
	\end{subfigure}
	\begin{subfigure}{.33\linewidth}
		\centering
		\includegraphics[width=0.99\linewidth]{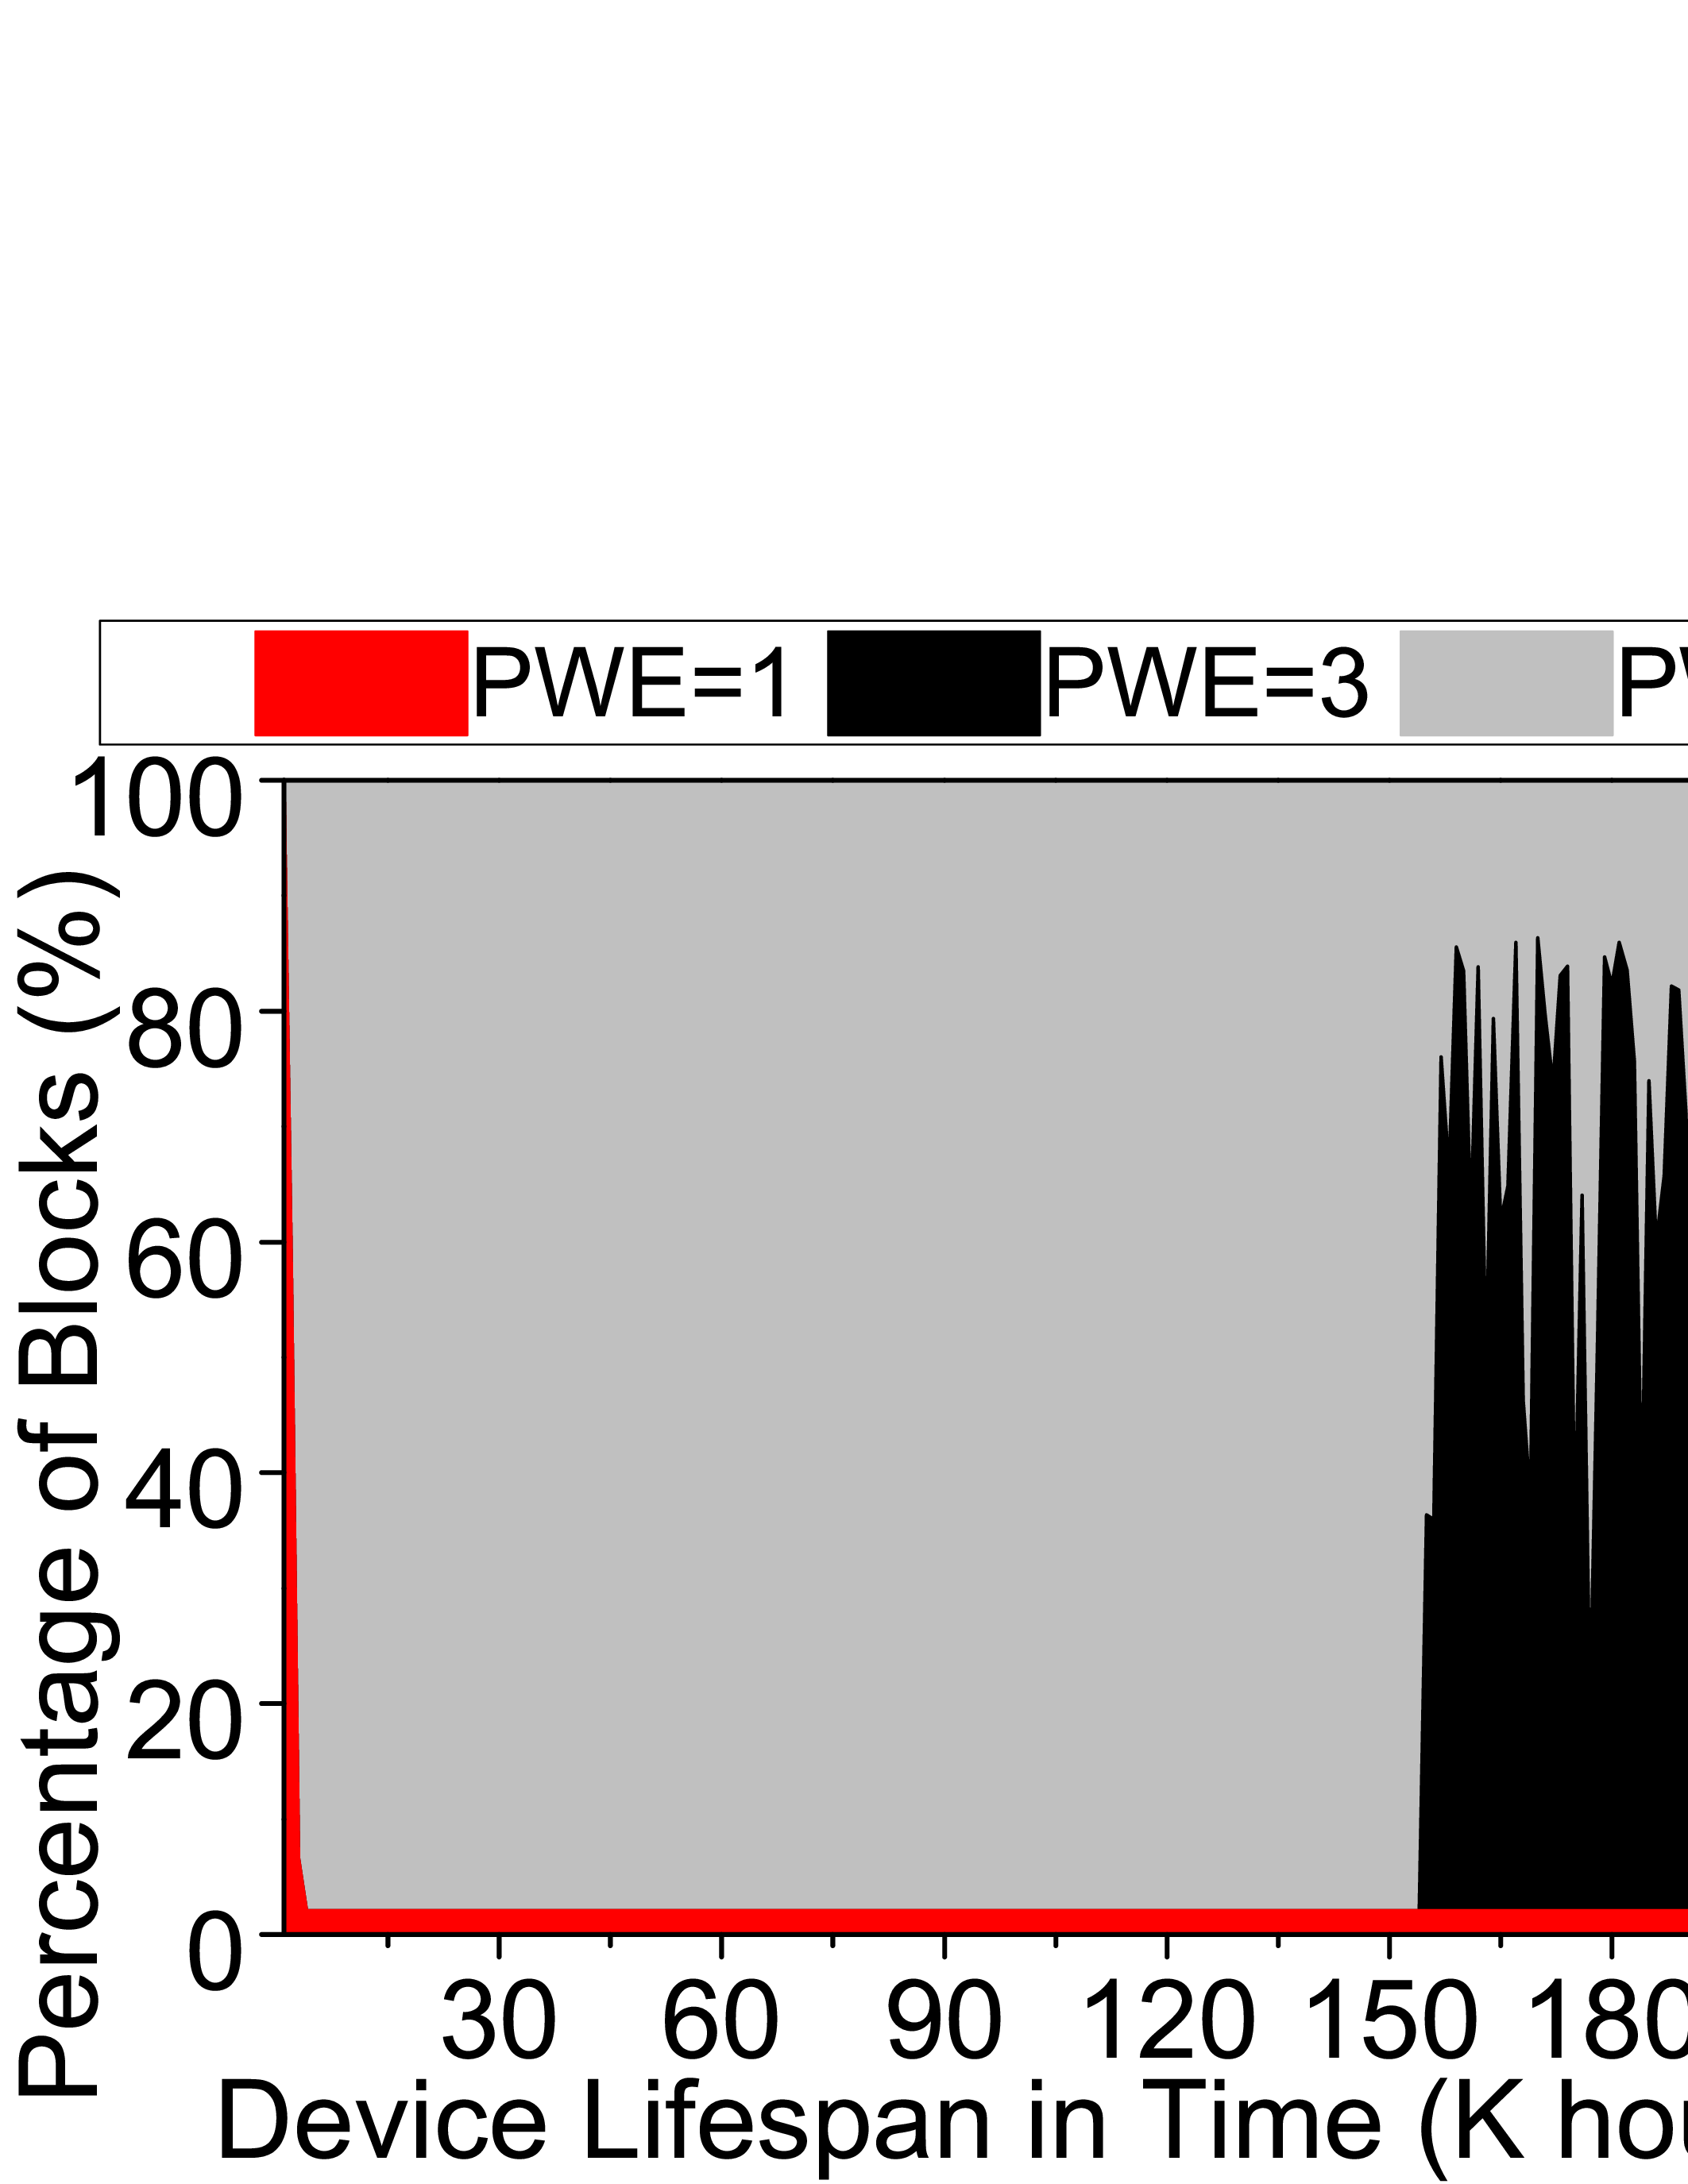}
		\caption{mds\textunderscore0 in Normal}\label{fig:pwe-sense-drift-mds_0-normal}
	\end{subfigure}
	\begin{subfigure}{.33\linewidth}
		\centering
		\includegraphics[width=0.99\linewidth]{graphs-app/pwe-mds_0-strong.eps}
		\caption{mds\textunderscore0 in Strong}\label{fig:pwe-sense-drift-mds_0-strong}
	\end{subfigure}
\caption{Percentages of blocks with 2, 4, and 8 states, when running \emph{mds\textunderscore0} on Weak, Normal, and Strong devices.}
\label{fig:pwe-sense-drift-mds_0}
\end{figure*}

\begin{figure*}
\centering
	\begin{subfigure}{.33\linewidth}
		\centering
		\includegraphics[width=0.99\linewidth]{graphs-app/pwe-src1_2-weak.eps}
		\caption{src1\textunderscore2 in Weak}\label{fig:pwe-sense-drift-src1_2-weak}
	\end{subfigure}
	\begin{subfigure}{.33\linewidth}
		\centering
		\includegraphics[width=0.99\linewidth]{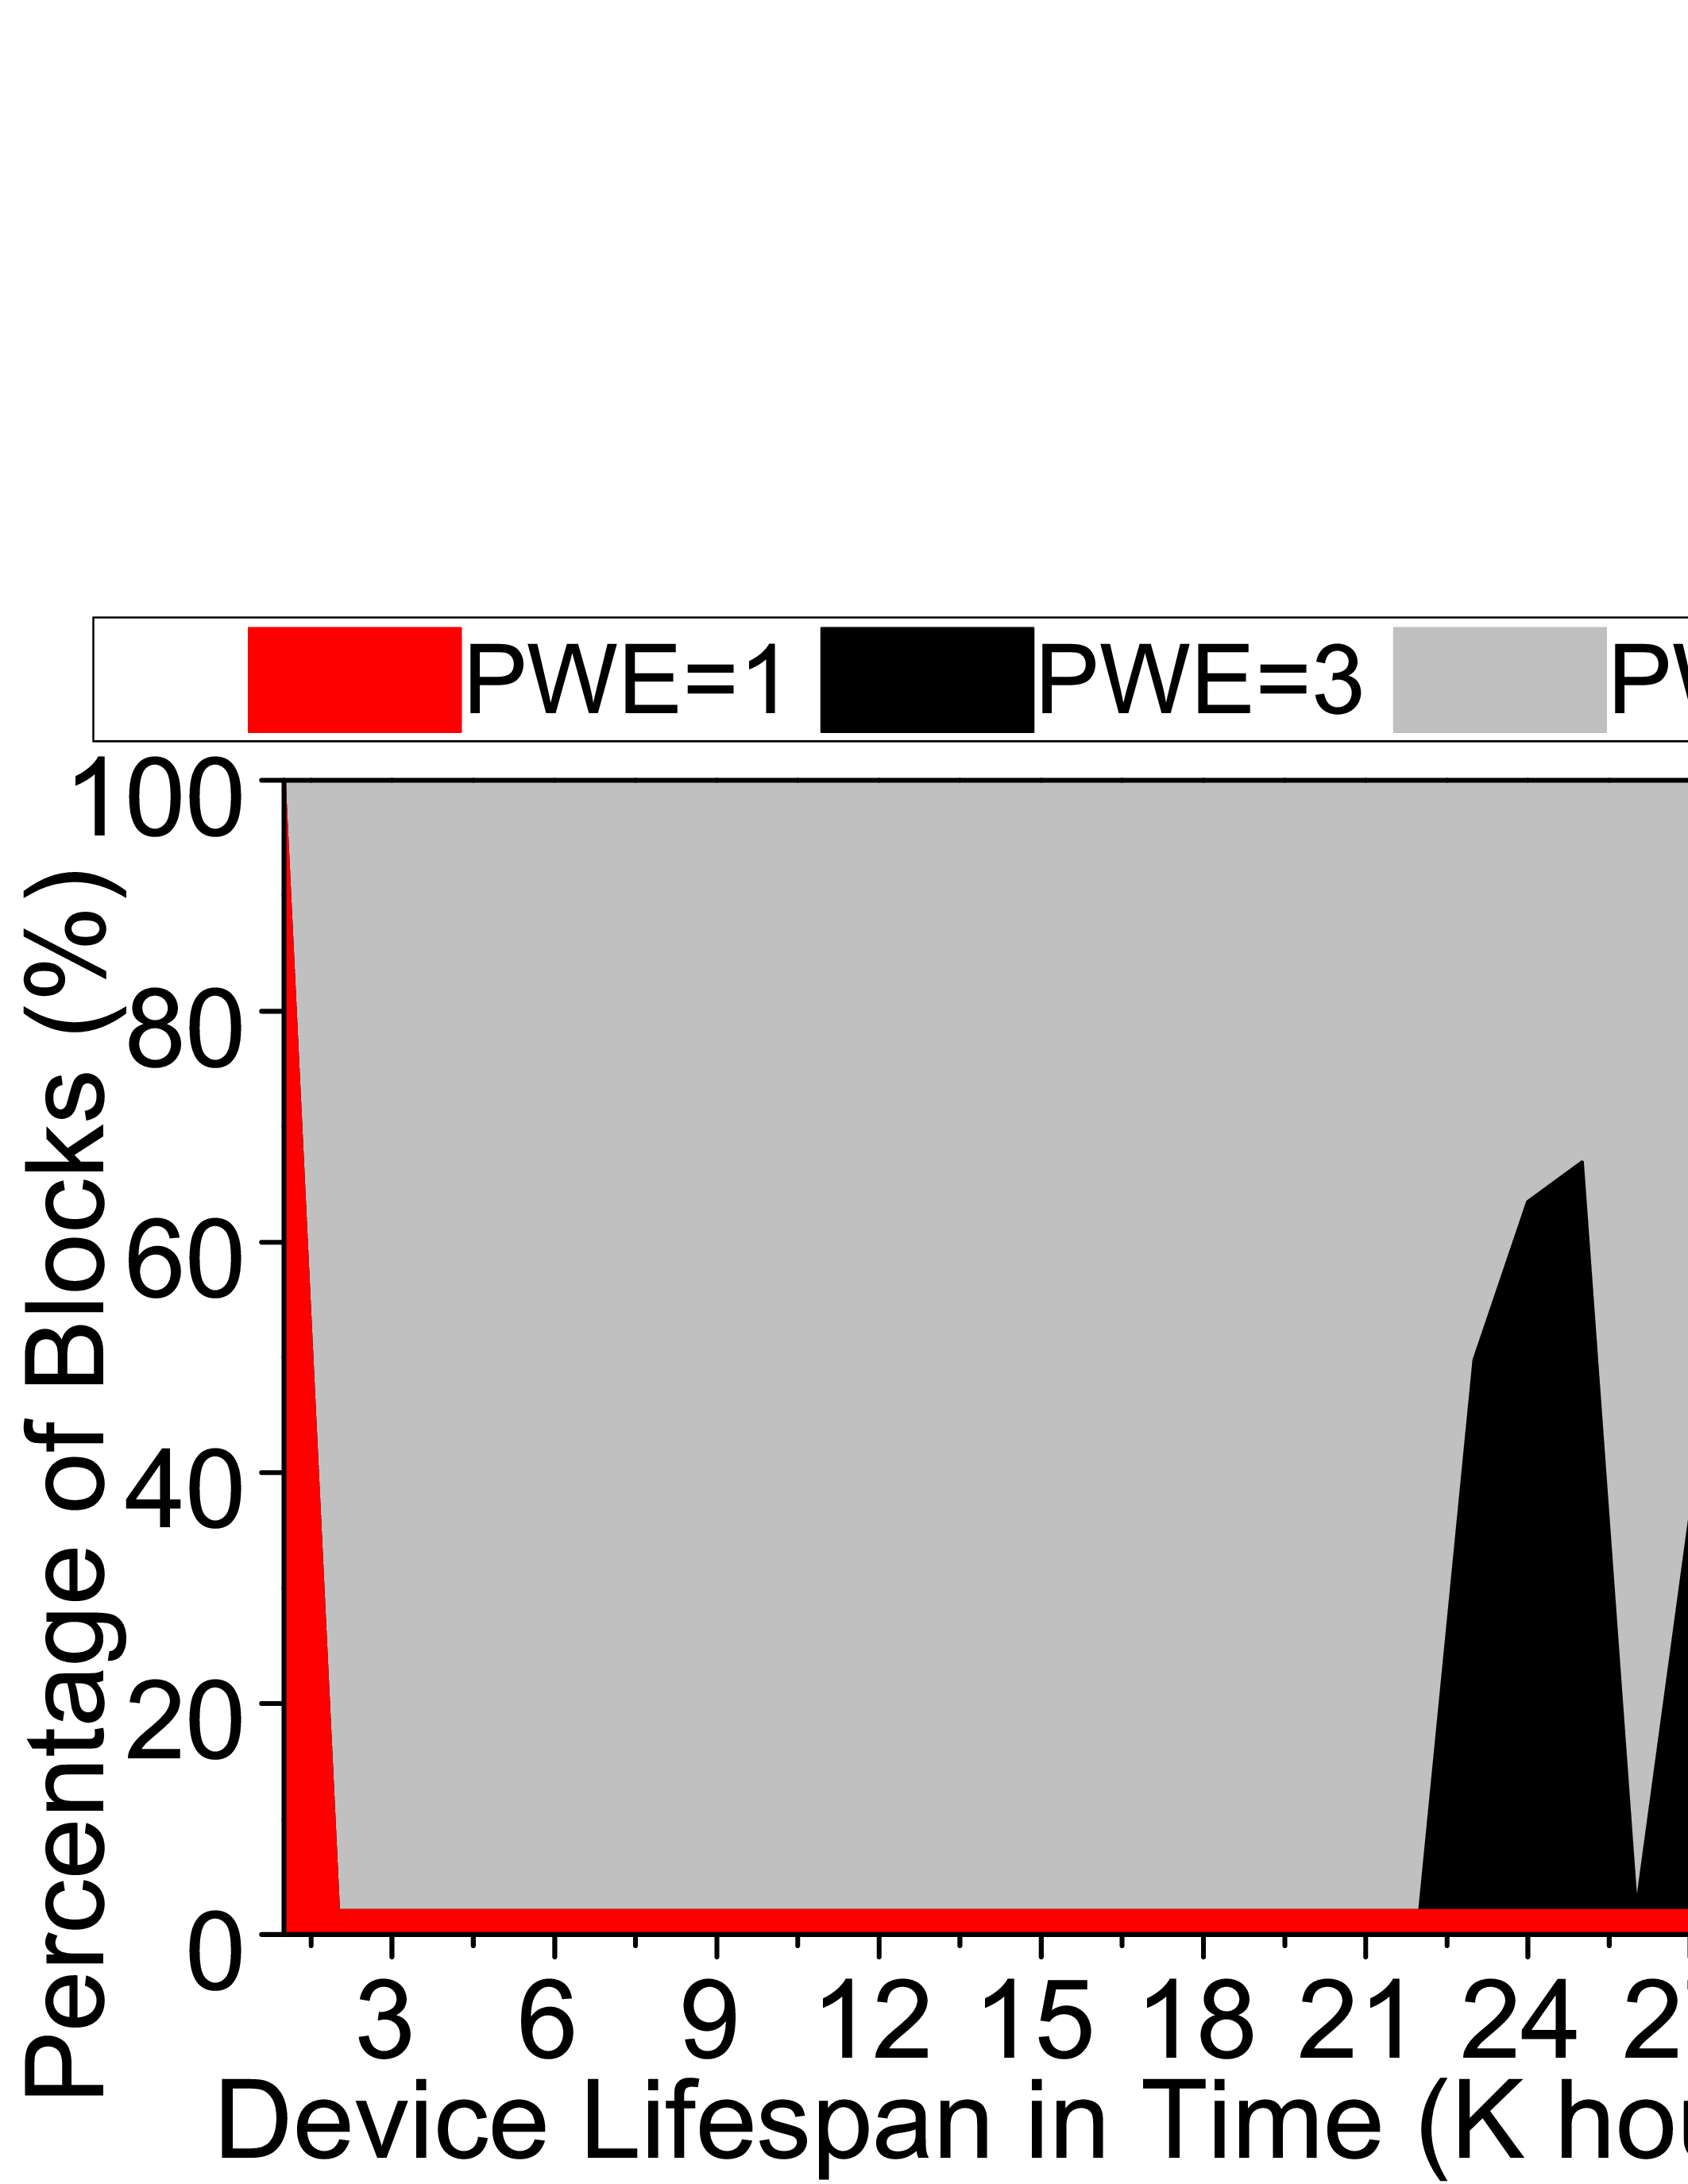}
		\caption{src1\textunderscore2 in Normal}\label{fig:pwe-sense-drift-src1_2-normal}
	\end{subfigure}
	\begin{subfigure}{.33\linewidth}
		\centering
		\includegraphics[width=0.99\linewidth]{graphs-app/pwe-src1_2-strong.eps}
		\caption{src1\textunderscore2 in Strong}\label{fig:pwe-sense-drift-src1_2-strong}
	\end{subfigure}
\caption{Percentages of blocks with 2, 4, and 8 states, when running \emph{src1\textunderscore2} on Weak, Normal, and Strong devices.}
\label{fig:pwe-sense-drift-src1_2}
\end{figure*}

\begin{figure*}
\centering
	\begin{subfigure}{.33\linewidth}
		\centering
		\includegraphics[width=0.99\linewidth]{graphs-app/pwe-src2_0-weak.eps}
		\caption{src2\textunderscore0 in Weak}\label{fig:pwe-sense-drift-src2_0-weak}
	\end{subfigure}
	\begin{subfigure}{.33\linewidth}
		\centering
		\includegraphics[width=0.99\linewidth]{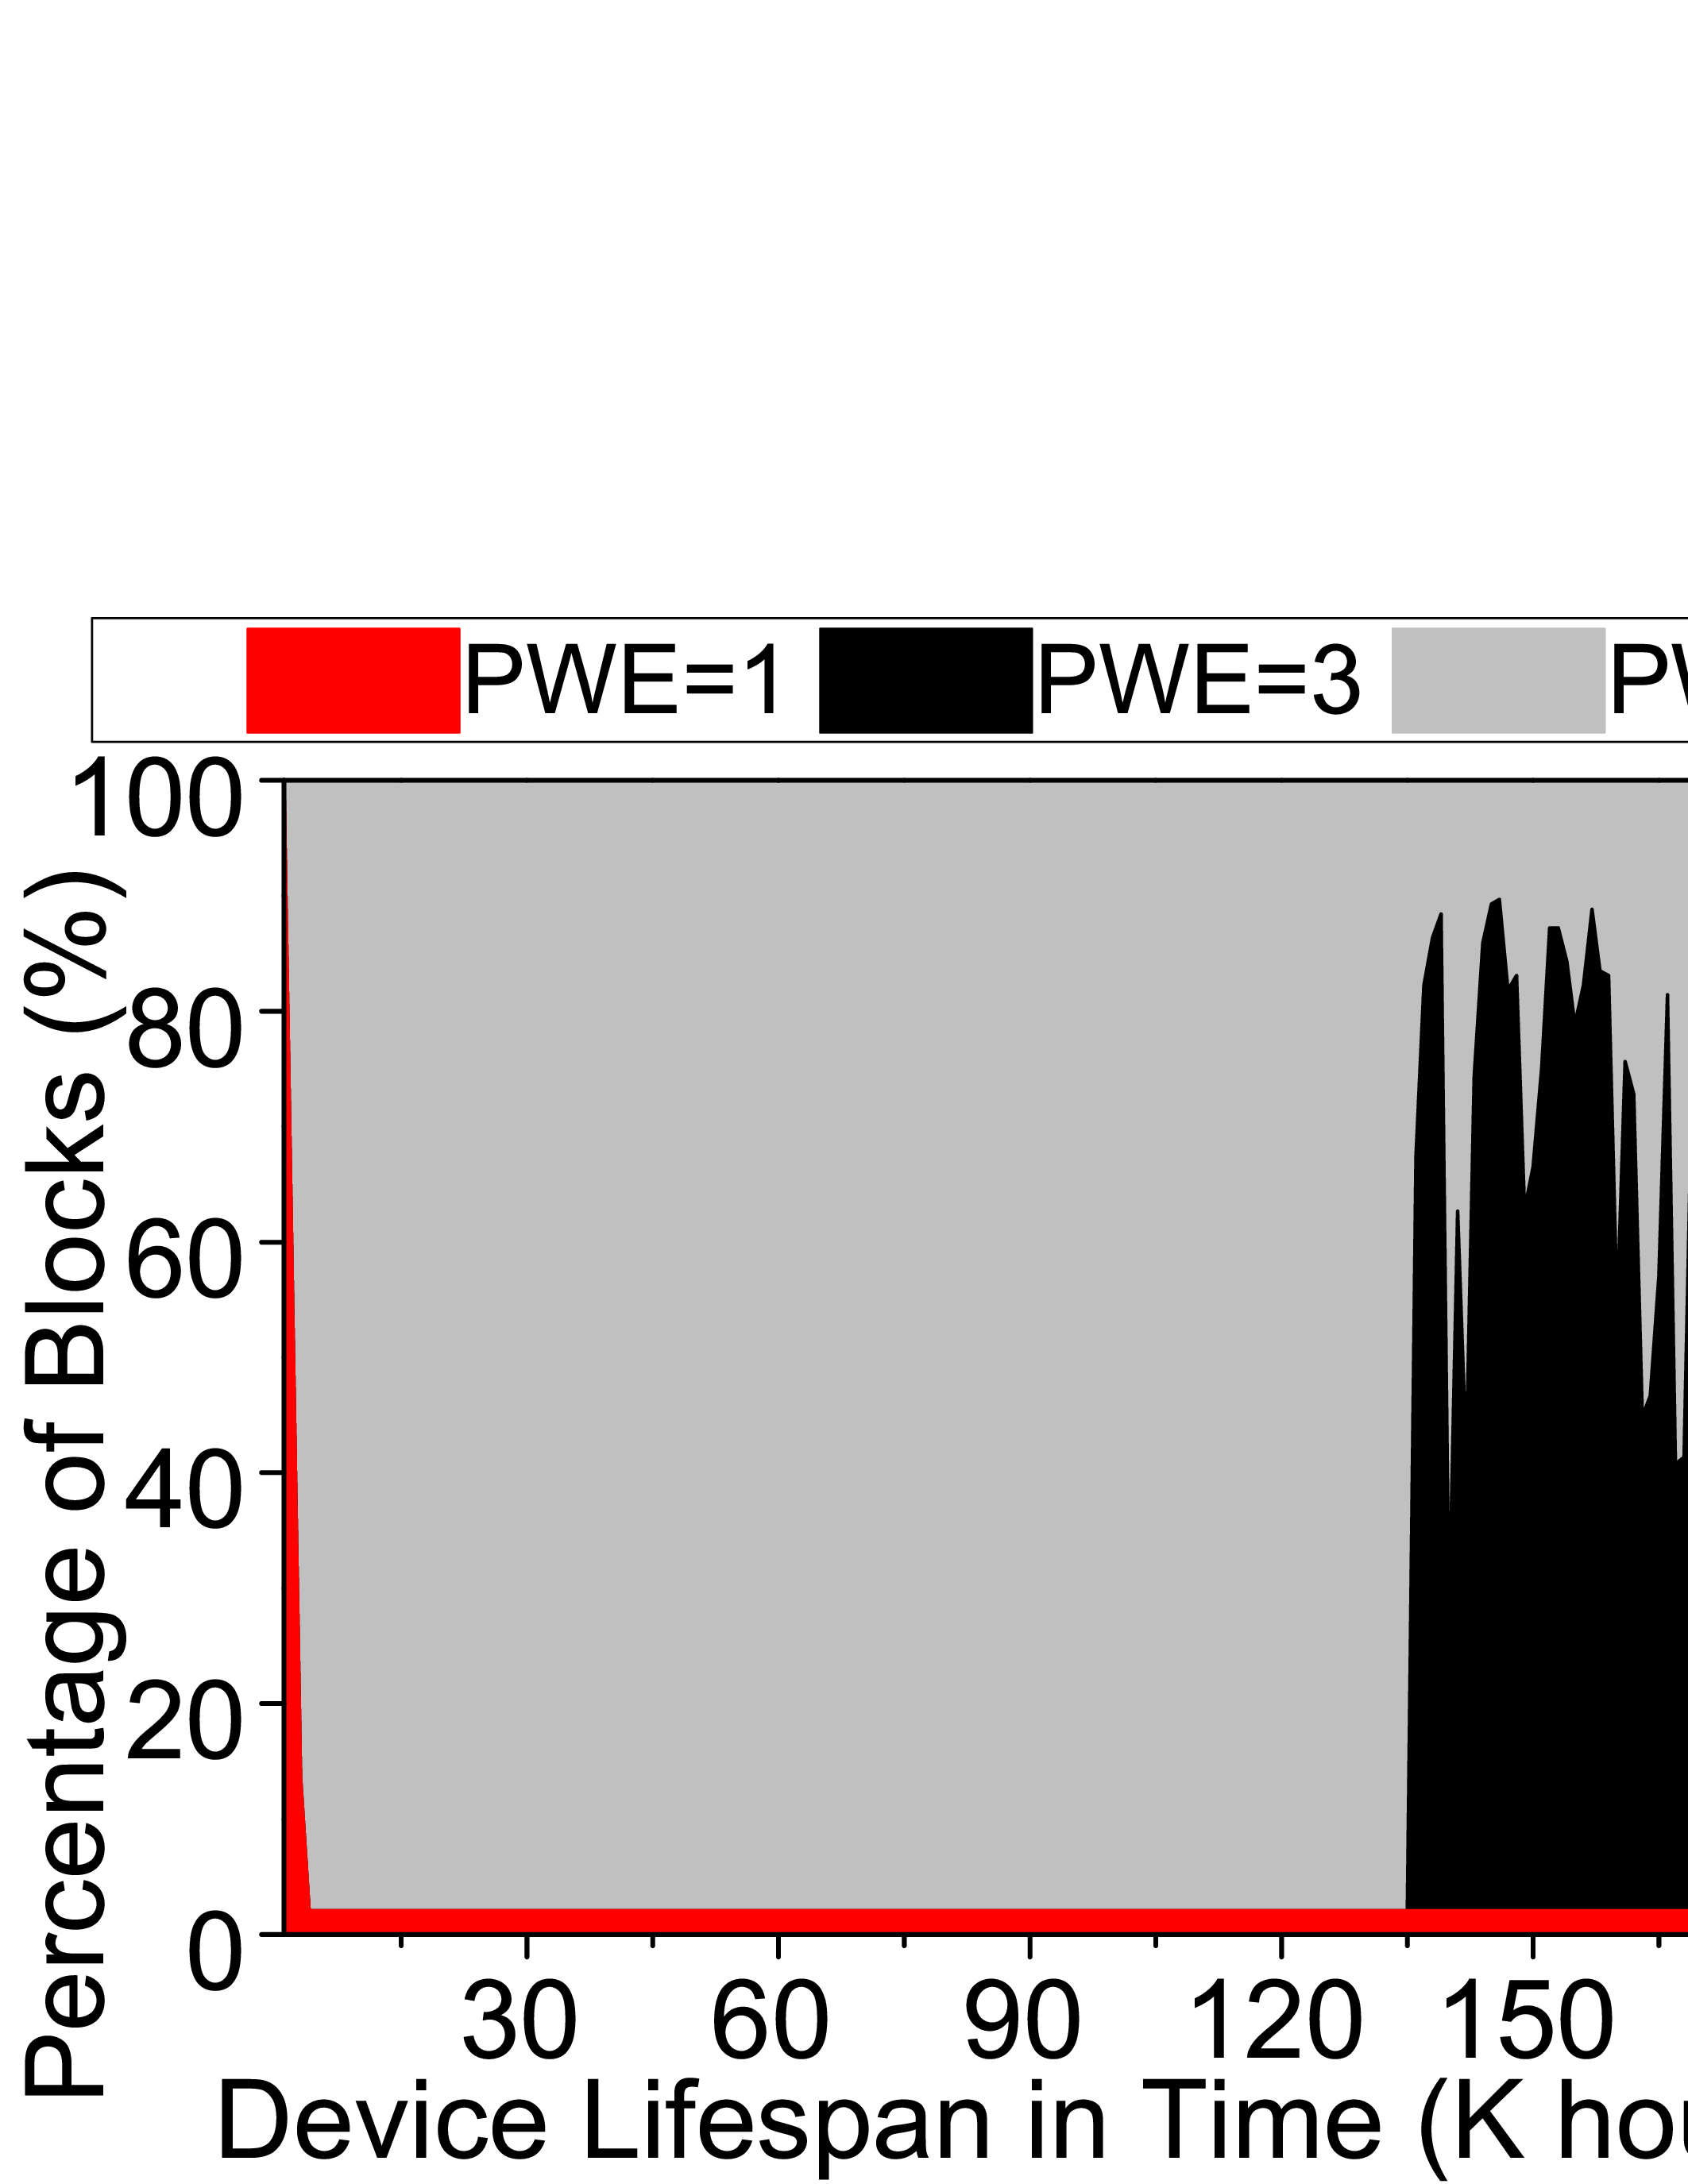}
		\caption{src2\textunderscore0 in Normal}\label{fig:pwe-sense-drift-src2_0-normal}
	\end{subfigure}
	\begin{subfigure}{.33\linewidth}
		\centering
		\includegraphics[width=0.99\linewidth]{graphs-app/pwe-src2_0-strong.eps}
		\caption{src2\textunderscore0 in Strong}\label{fig:pwe-sense-drift-src2_0-strong}
	\end{subfigure}
\caption{Percentages of blocks with 2, 4, and 8 states, when running \emph{src2\textunderscore0} on Weak, Normal, and Strong devices.}
\label{fig:pwe-sense-drift-src2_0}
\end{figure*}

\begin{figure*}
\centering
	\begin{subfigure}{.33\linewidth}
		\centering
		\includegraphics[width=0.99\linewidth]{graphs-app/pwe-stg_0-weak.eps}
		\caption{stg\textunderscore0 in Weak}\label{fig:pwe-sense-drift-stg_0-weak}
	\end{subfigure}
	\begin{subfigure}{.33\linewidth}
		\centering
		\includegraphics[width=0.99\linewidth]{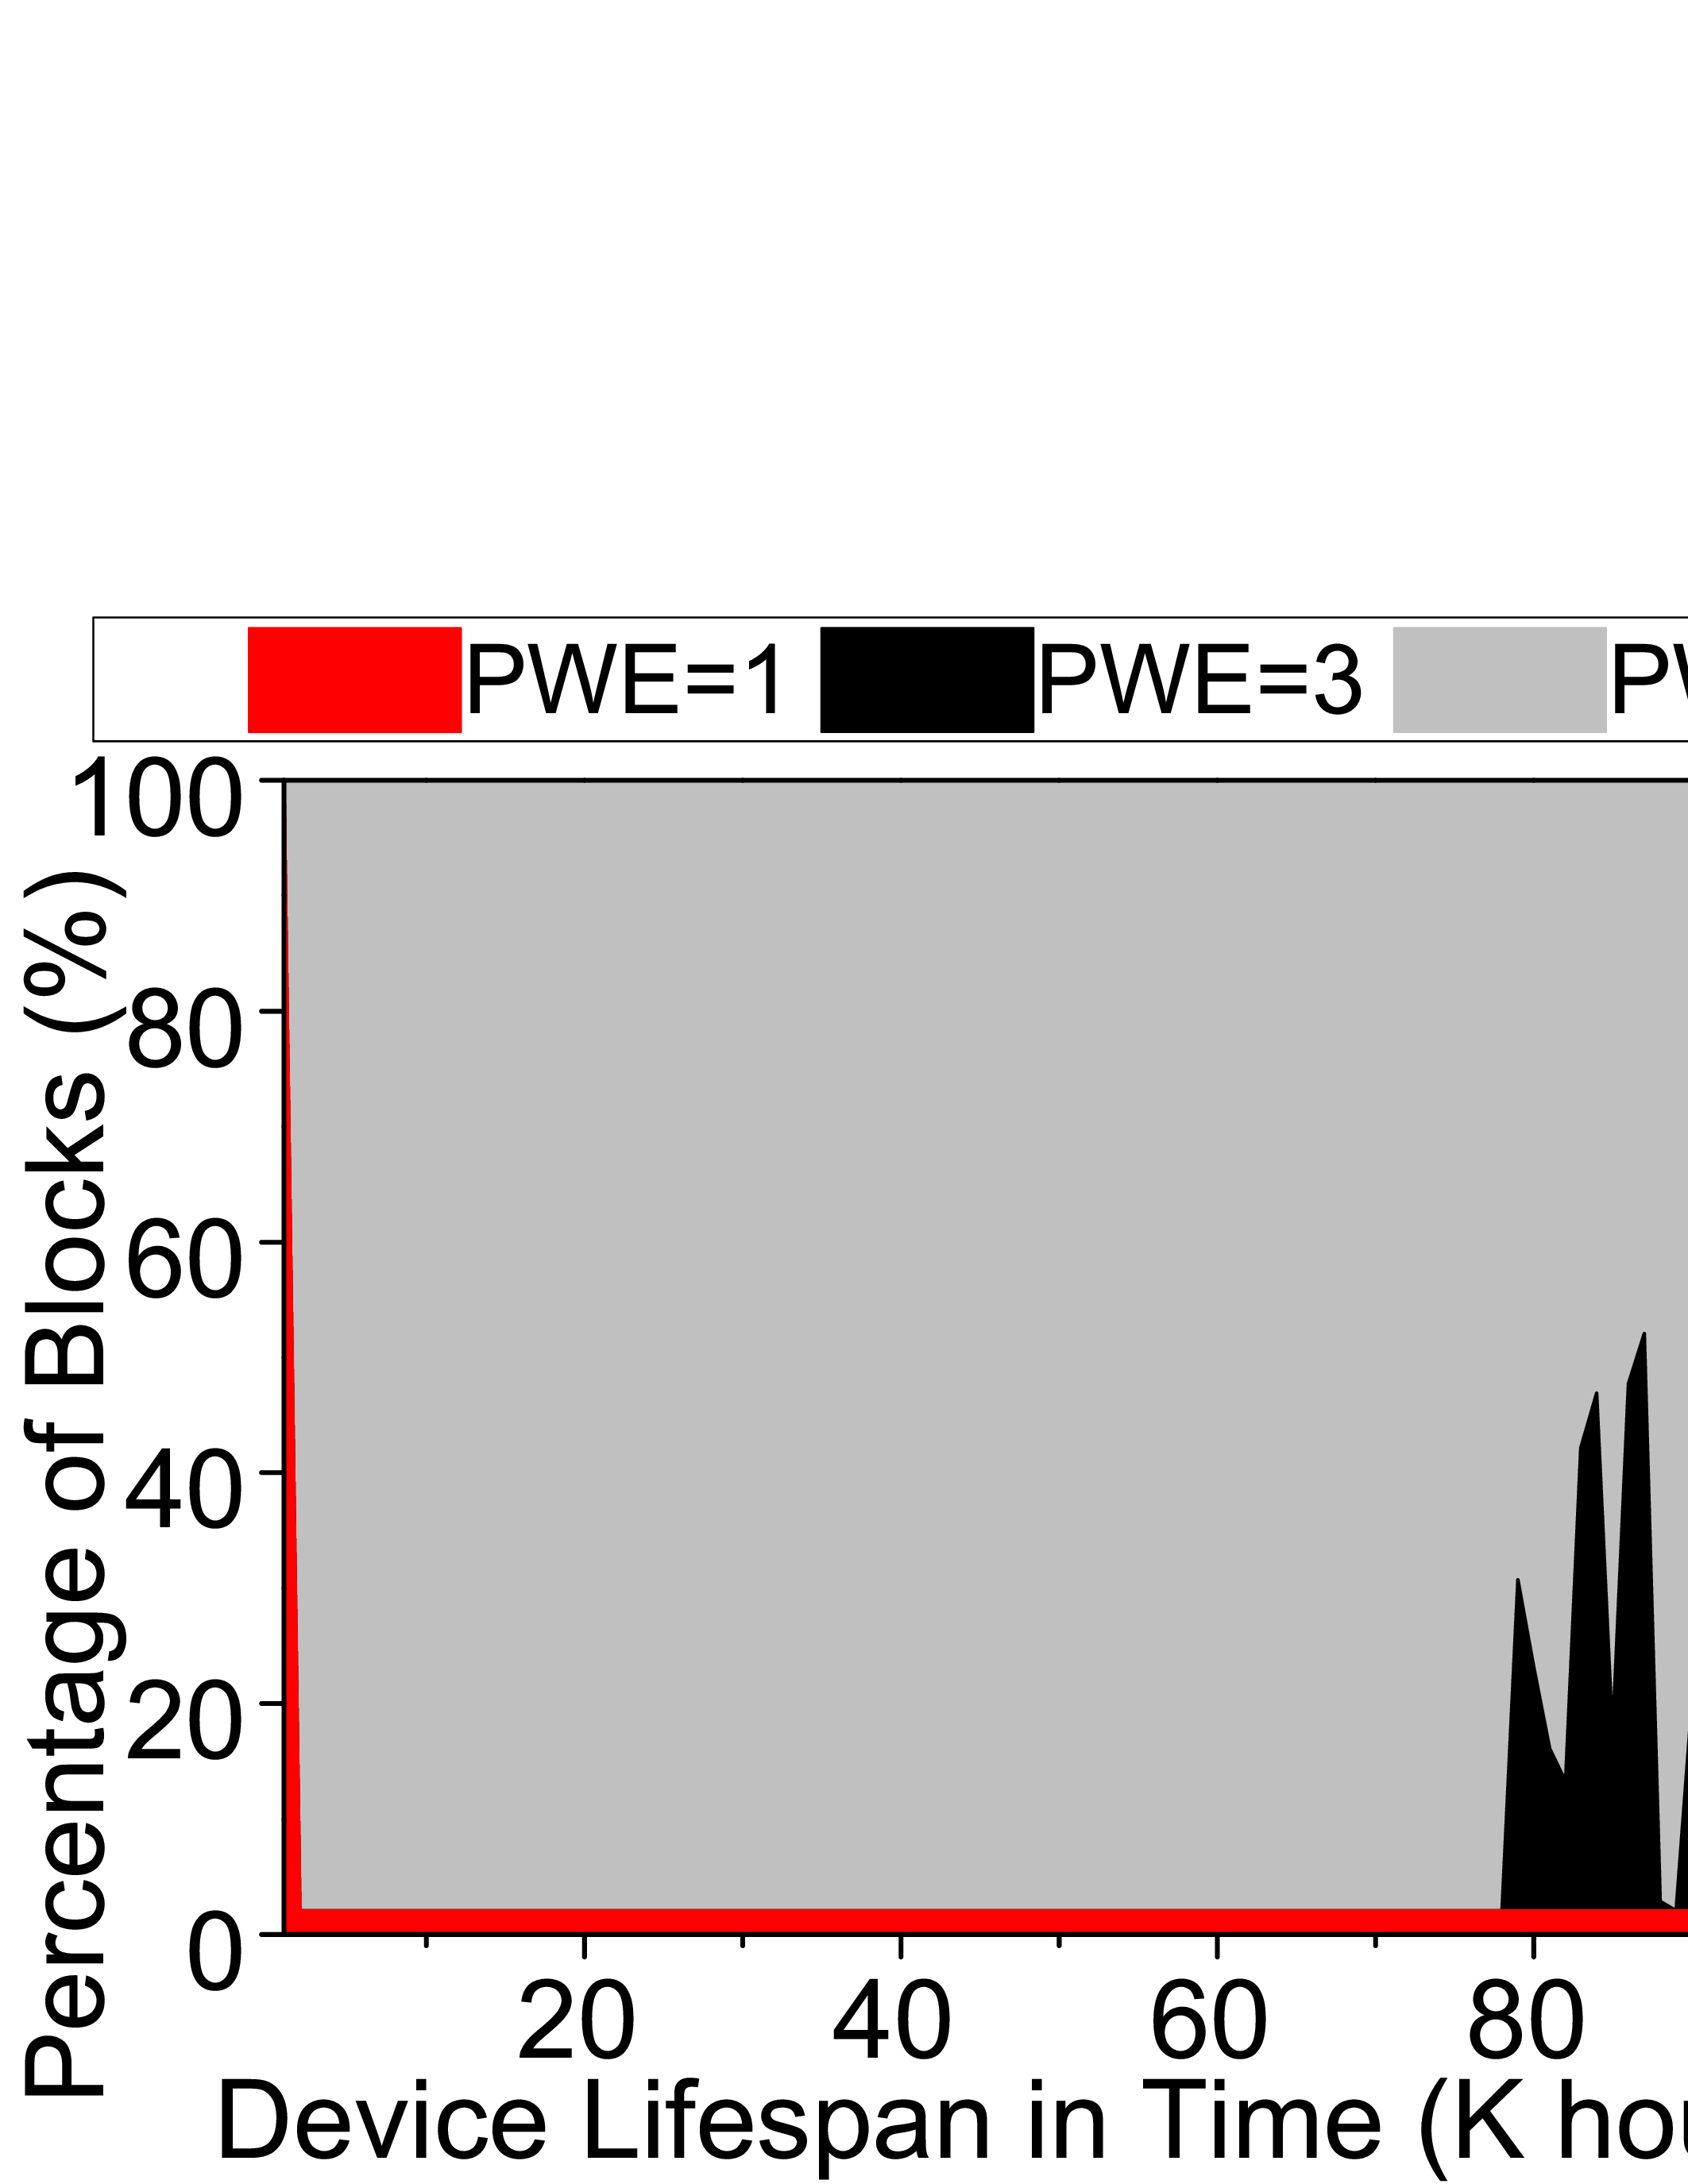}
		\caption{stg\textunderscore0 in Normal}\label{fig:pwe-sense-drift-stg_0-normal}
	\end{subfigure}
	\begin{subfigure}{.33\linewidth}
		\centering
		\includegraphics[width=0.99\linewidth]{graphs-app/pwe-stg_0-strong.eps}
		\caption{stg\textunderscore0 in Strong}\label{fig:pwe-sense-drift-stg_0-strong}
	\end{subfigure}
\caption{Percentages of blocks with 2, 4, and 8 states, when running \emph{stg\textunderscore0} on Weak, Normal, and Strong devices.}
\label{fig:pwe-sense-drift-stg_0}
\end{figure*}

\begin{figure*}
\centering
	\begin{subfigure}{.33\linewidth}
		\centering
		\includegraphics[width=0.99\linewidth]{graphs-app/pwe-usr_0-weak.eps}
		\caption{usr\textunderscore0 in Weak}\label{fig:pwe-sense-drift-usr_0-weak}
	\end{subfigure}
	\begin{subfigure}{.33\linewidth}
		\centering
		\includegraphics[width=0.99\linewidth]{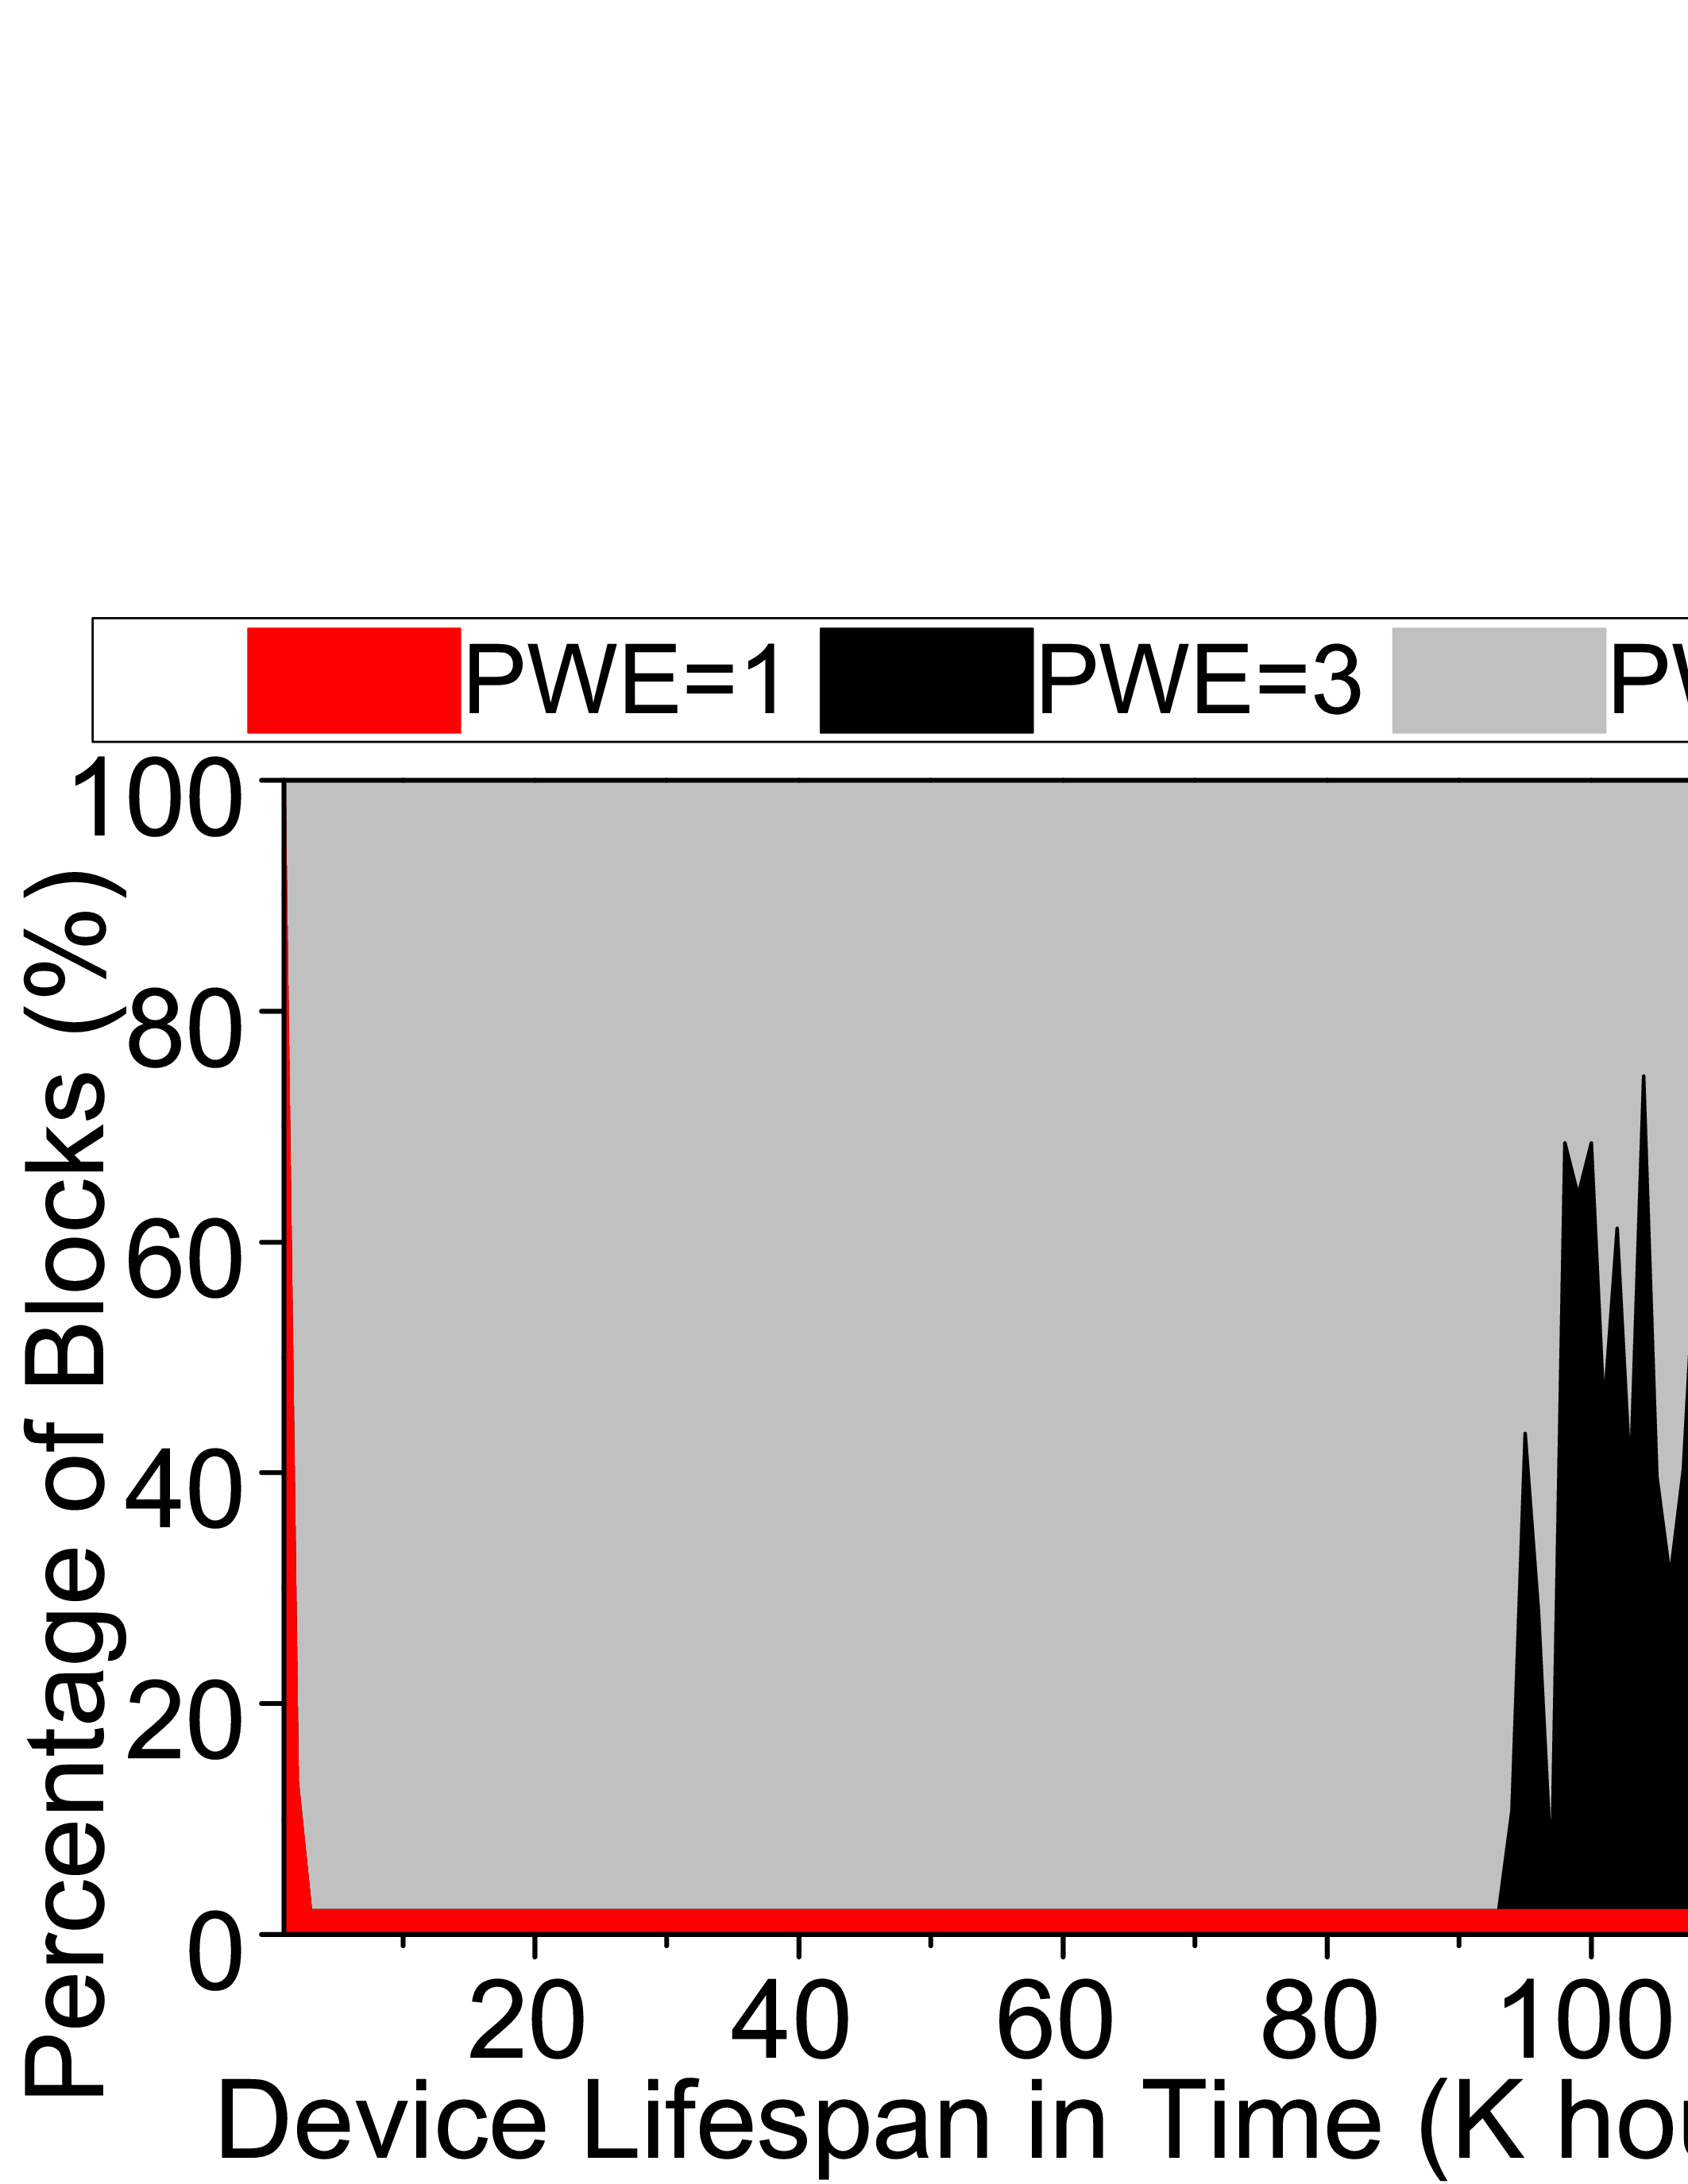}
		\caption{usr\textunderscore0 in Normal}\label{fig:pwe-sense-drift-usr_0-normal}
	\end{subfigure}
	\begin{subfigure}{.33\linewidth}
		\centering
		\includegraphics[width=0.99\linewidth]{graphs-app/pwe-usr_0-strong.eps}
		\caption{usr\textunderscore0 in Strong}\label{fig:pwe-sense-drift-usr_0-strong}
	\end{subfigure}
\caption{Percentages of blocks with 2, 4, and 8 states, when running \emph{usr\textunderscore0} on Weak, Normal, and Strong devices.}
\label{fig:pwe-sense-drift-usr_0}
\end{figure*}

\begin{figure*}
\centering
	\begin{subfigure}{.33\linewidth}
		\centering
		\includegraphics[width=0.99\linewidth]{graphs-app/pwe-web_0-weak.eps}
		\caption{web\textunderscore0 in Weak}\label{fig:pwe-sense-drift-web_0-weak}
	\end{subfigure}
	\begin{subfigure}{.33\linewidth}
		\centering
		\includegraphics[width=0.99\linewidth]{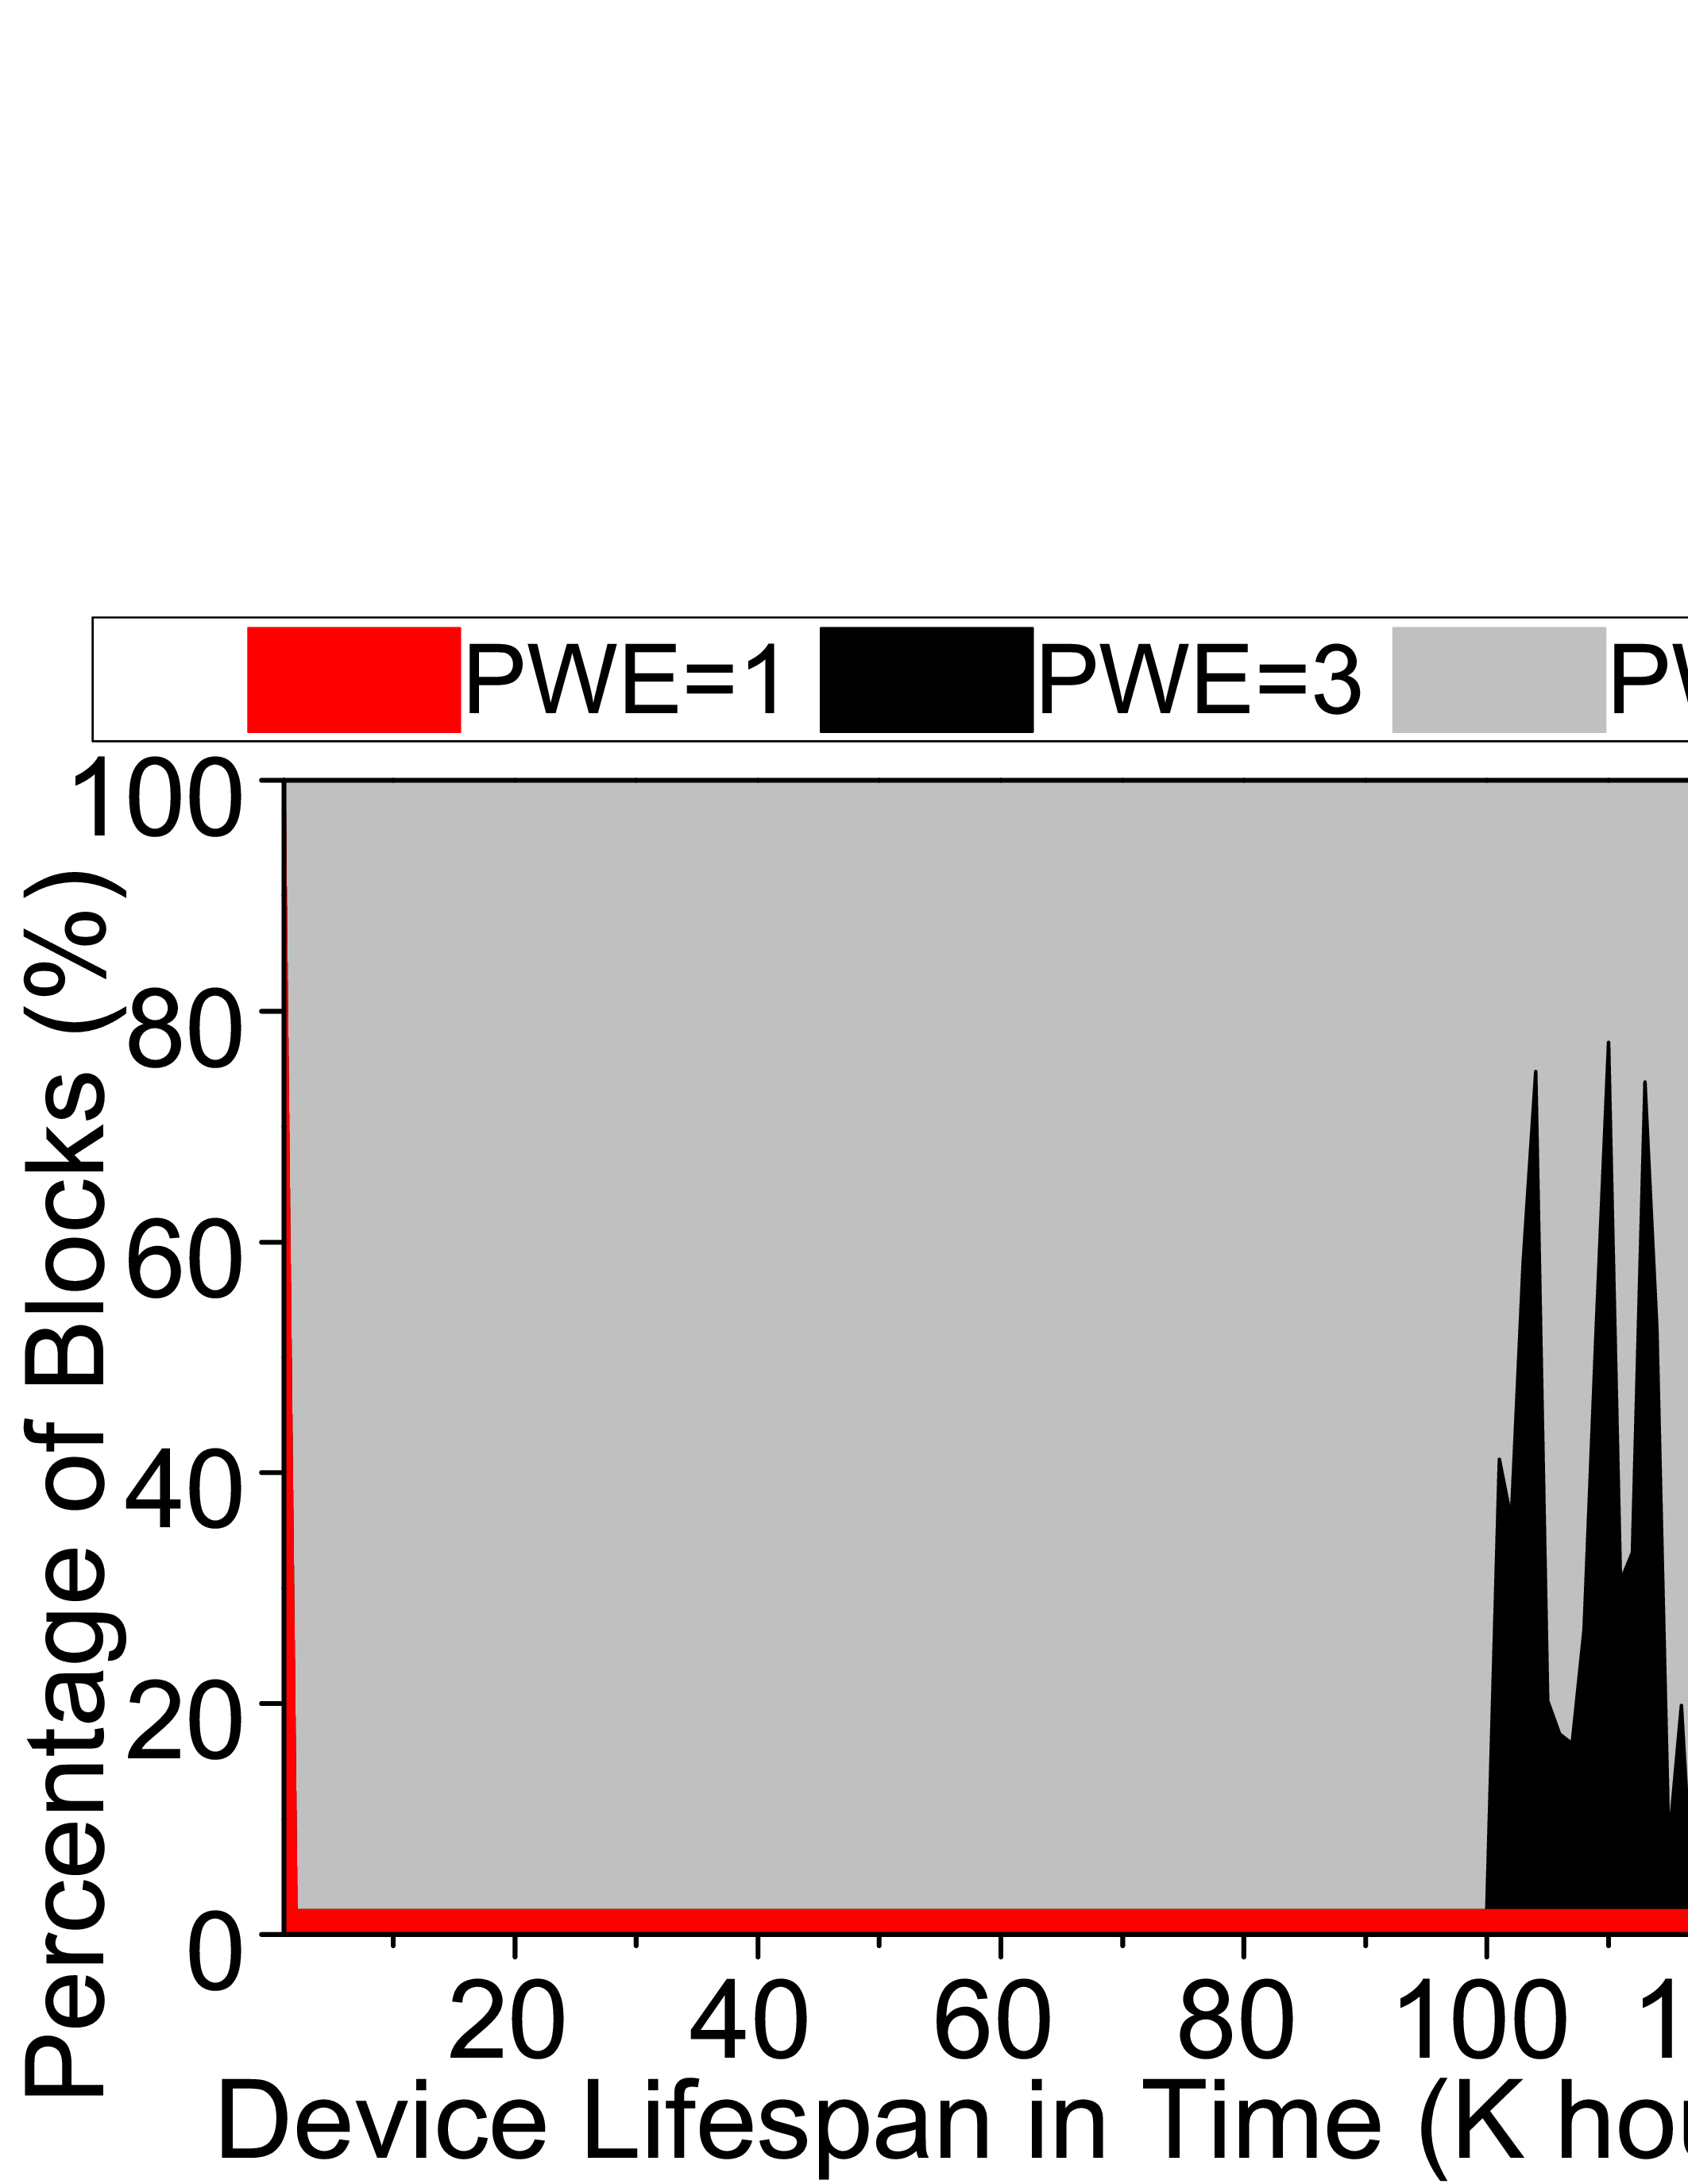}
		\caption{web\textunderscore0 in Normal}\label{fig:pwe-sense-drift-web_0-normal}
	\end{subfigure}
	\begin{subfigure}{.33\linewidth}
		\centering
		\includegraphics[width=0.99\linewidth]{graphs-app/pwe-web_0-strong.eps}
		\caption{web\textunderscore0 in Strong}\label{fig:pwe-sense-drift-web_0-strong}
	\end{subfigure}
\caption{Percentages of blocks with 2, 4, and 8 states, when running \emph{web\textunderscore0} on Weak, Normal, and Strong devices.}
\label{fig:pwe-sense-drift-web_0}
\end{figure*}

\begin{figure*}
\centering
	\begin{subfigure}{.33\linewidth}
		\centering
		\includegraphics[width=0.99\linewidth]{graphs-app/pwe-wdev_0-weak.eps}
		\caption{wdev\textunderscore0 in Weak}\label{fig:pwe-sense-drift-wdev_0-weak}
	\end{subfigure}
	\begin{subfigure}{.33\linewidth}
		\centering
		\includegraphics[width=0.99\linewidth]{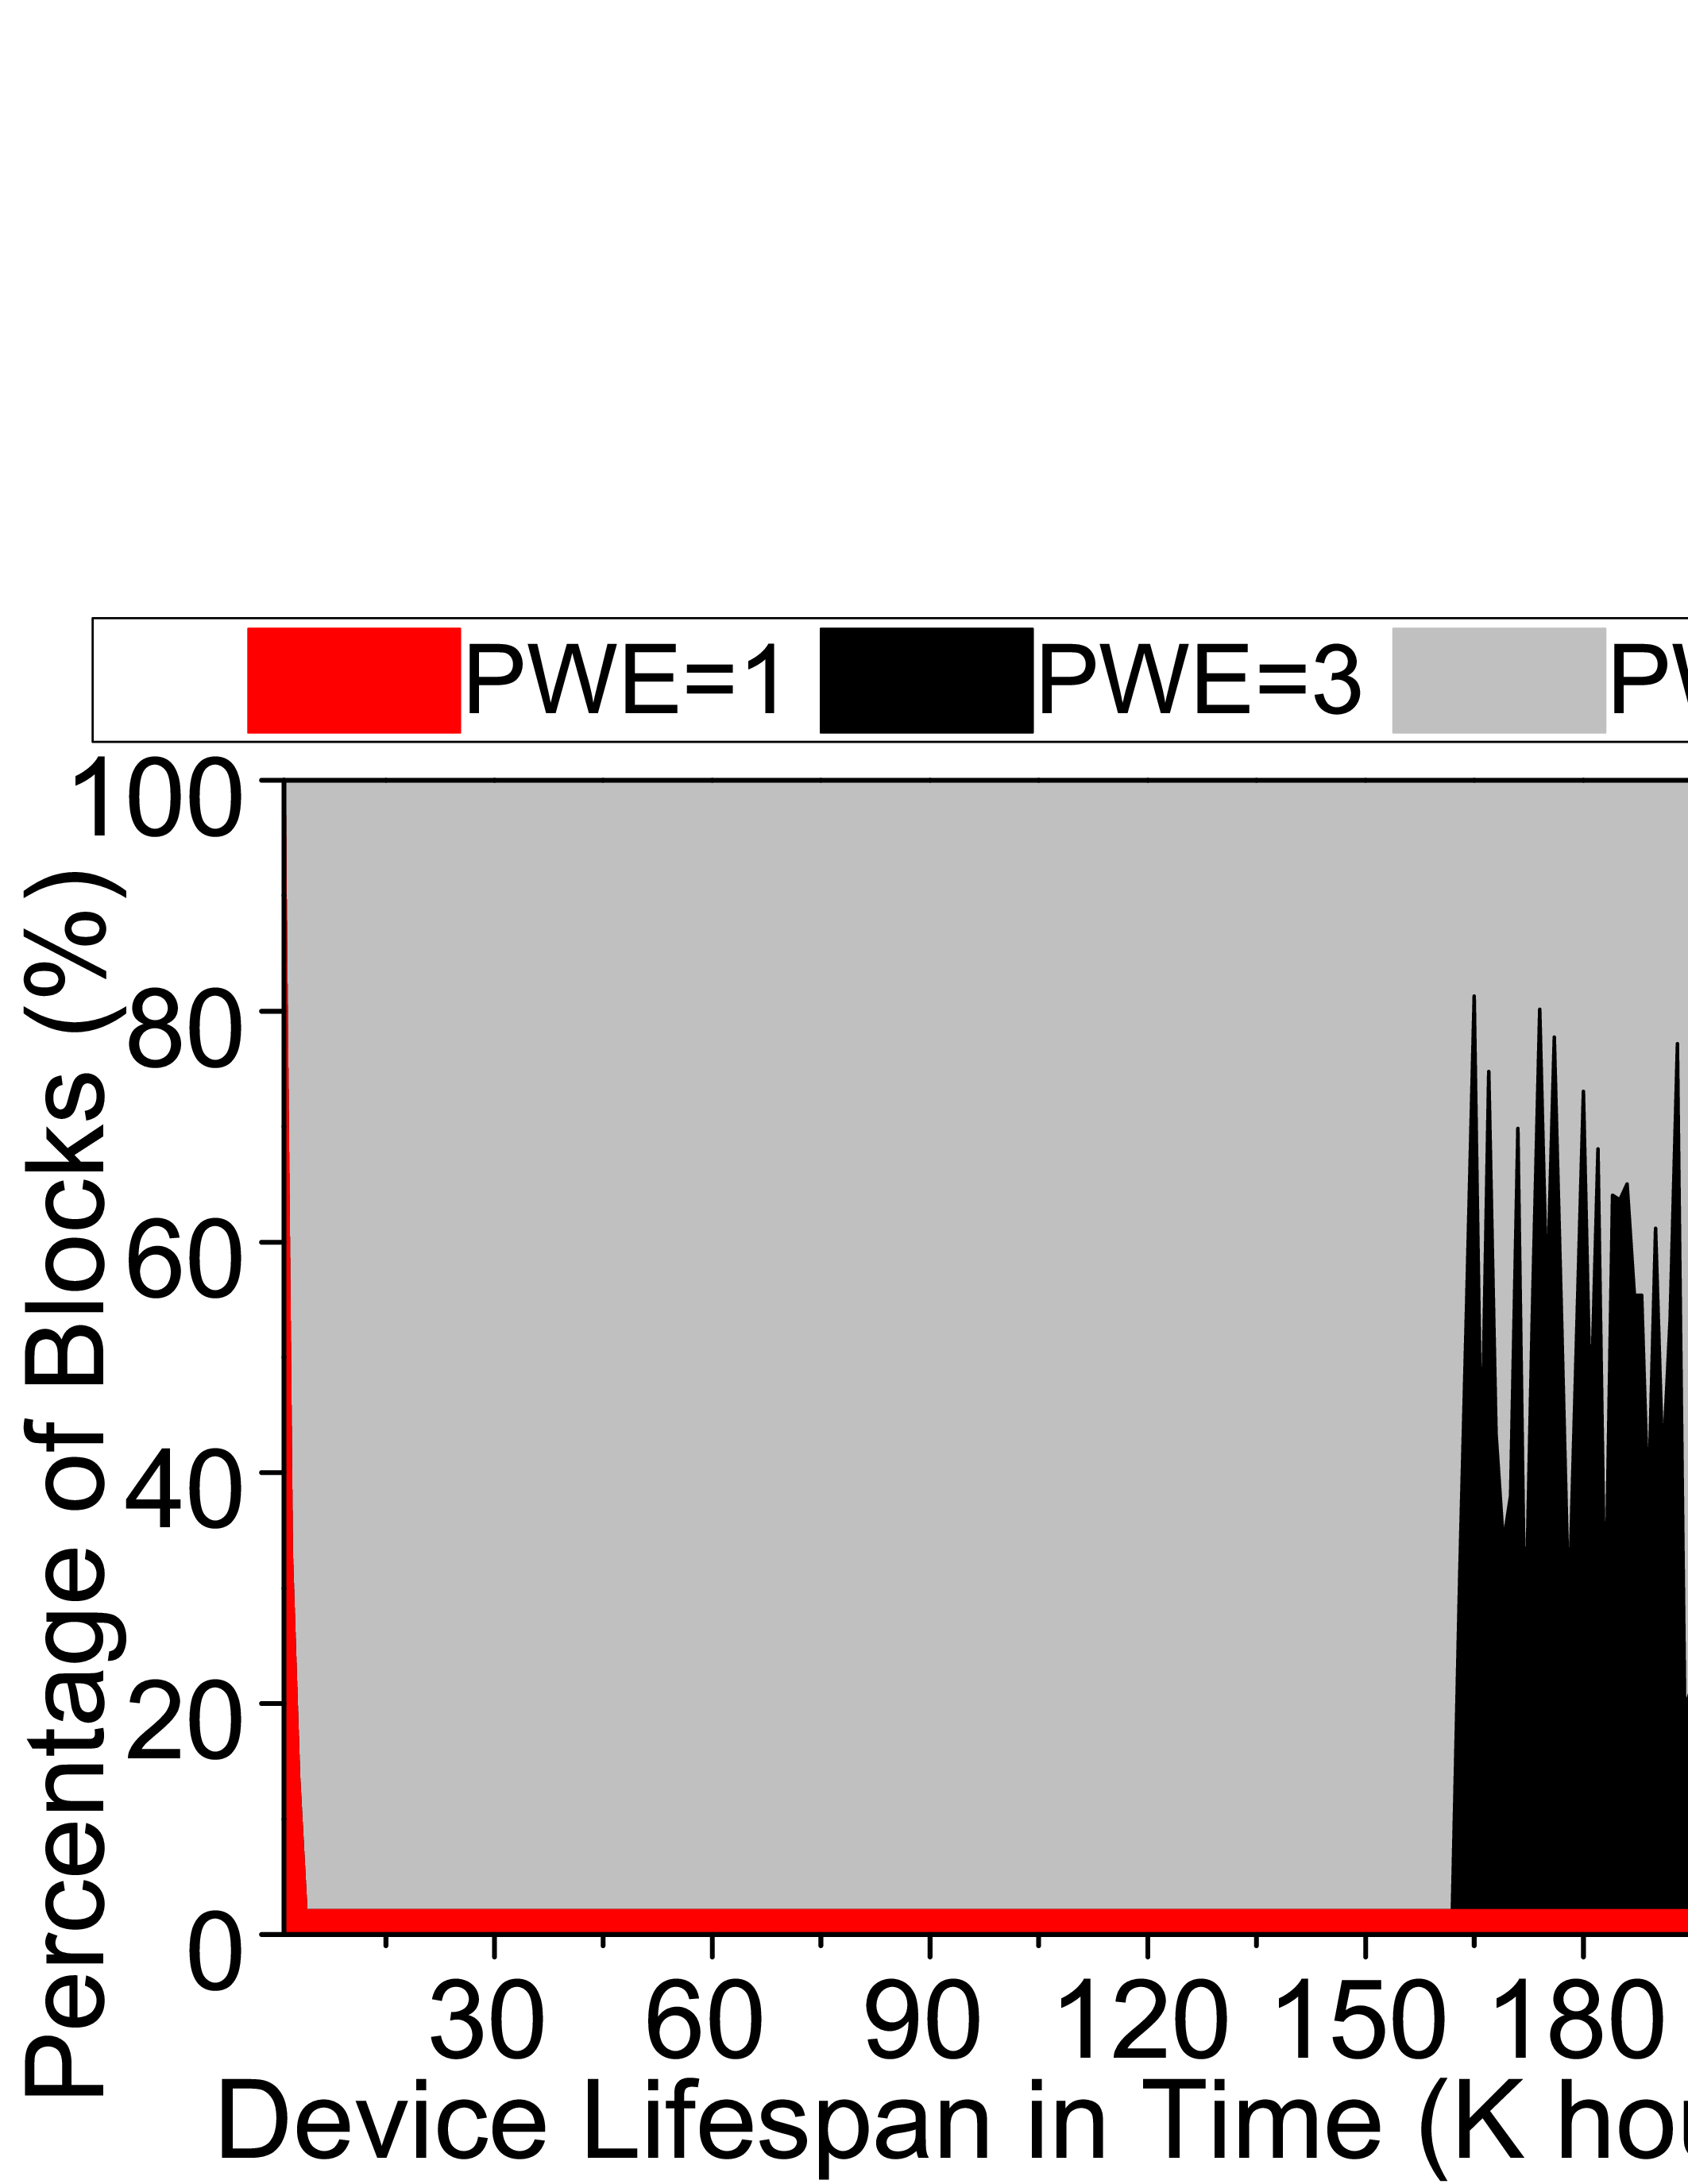}
		\caption{wdev\textunderscore0 in Normal}\label{fig:pwe-sense-drift-wdev_0-normal}
	\end{subfigure}
	\begin{subfigure}{.33\linewidth}
		\centering
		\includegraphics[width=0.99\linewidth]{graphs-app/pwe-wdev_0-strong.eps}
		\caption{wdev\textunderscore0 in Strong}\label{fig:pwe-sense-drift-wdev_0-strong}
	\end{subfigure}
\caption{Percentages of blocks with 2, 4, and 8 states, when running \emph{wdev\textunderscore0} on Weak, Normal, and Strong devices.}
\label{fig:pwe-sense-drift-wdev_0}
\end{figure*}

\begin{figure*}
\centering
	\begin{subfigure}{.33\linewidth}
		\centering
		\includegraphics[width=0.99\linewidth]{graphs-app/pwe-wdev_2-weak.eps}
		\caption{wdev\textunderscore2 in Weak}\label{fig:pwe-sense-drift-wdev_2-weak}
	\end{subfigure}
	\begin{subfigure}{.33\linewidth}
		\centering
		\includegraphics[width=0.99\linewidth]{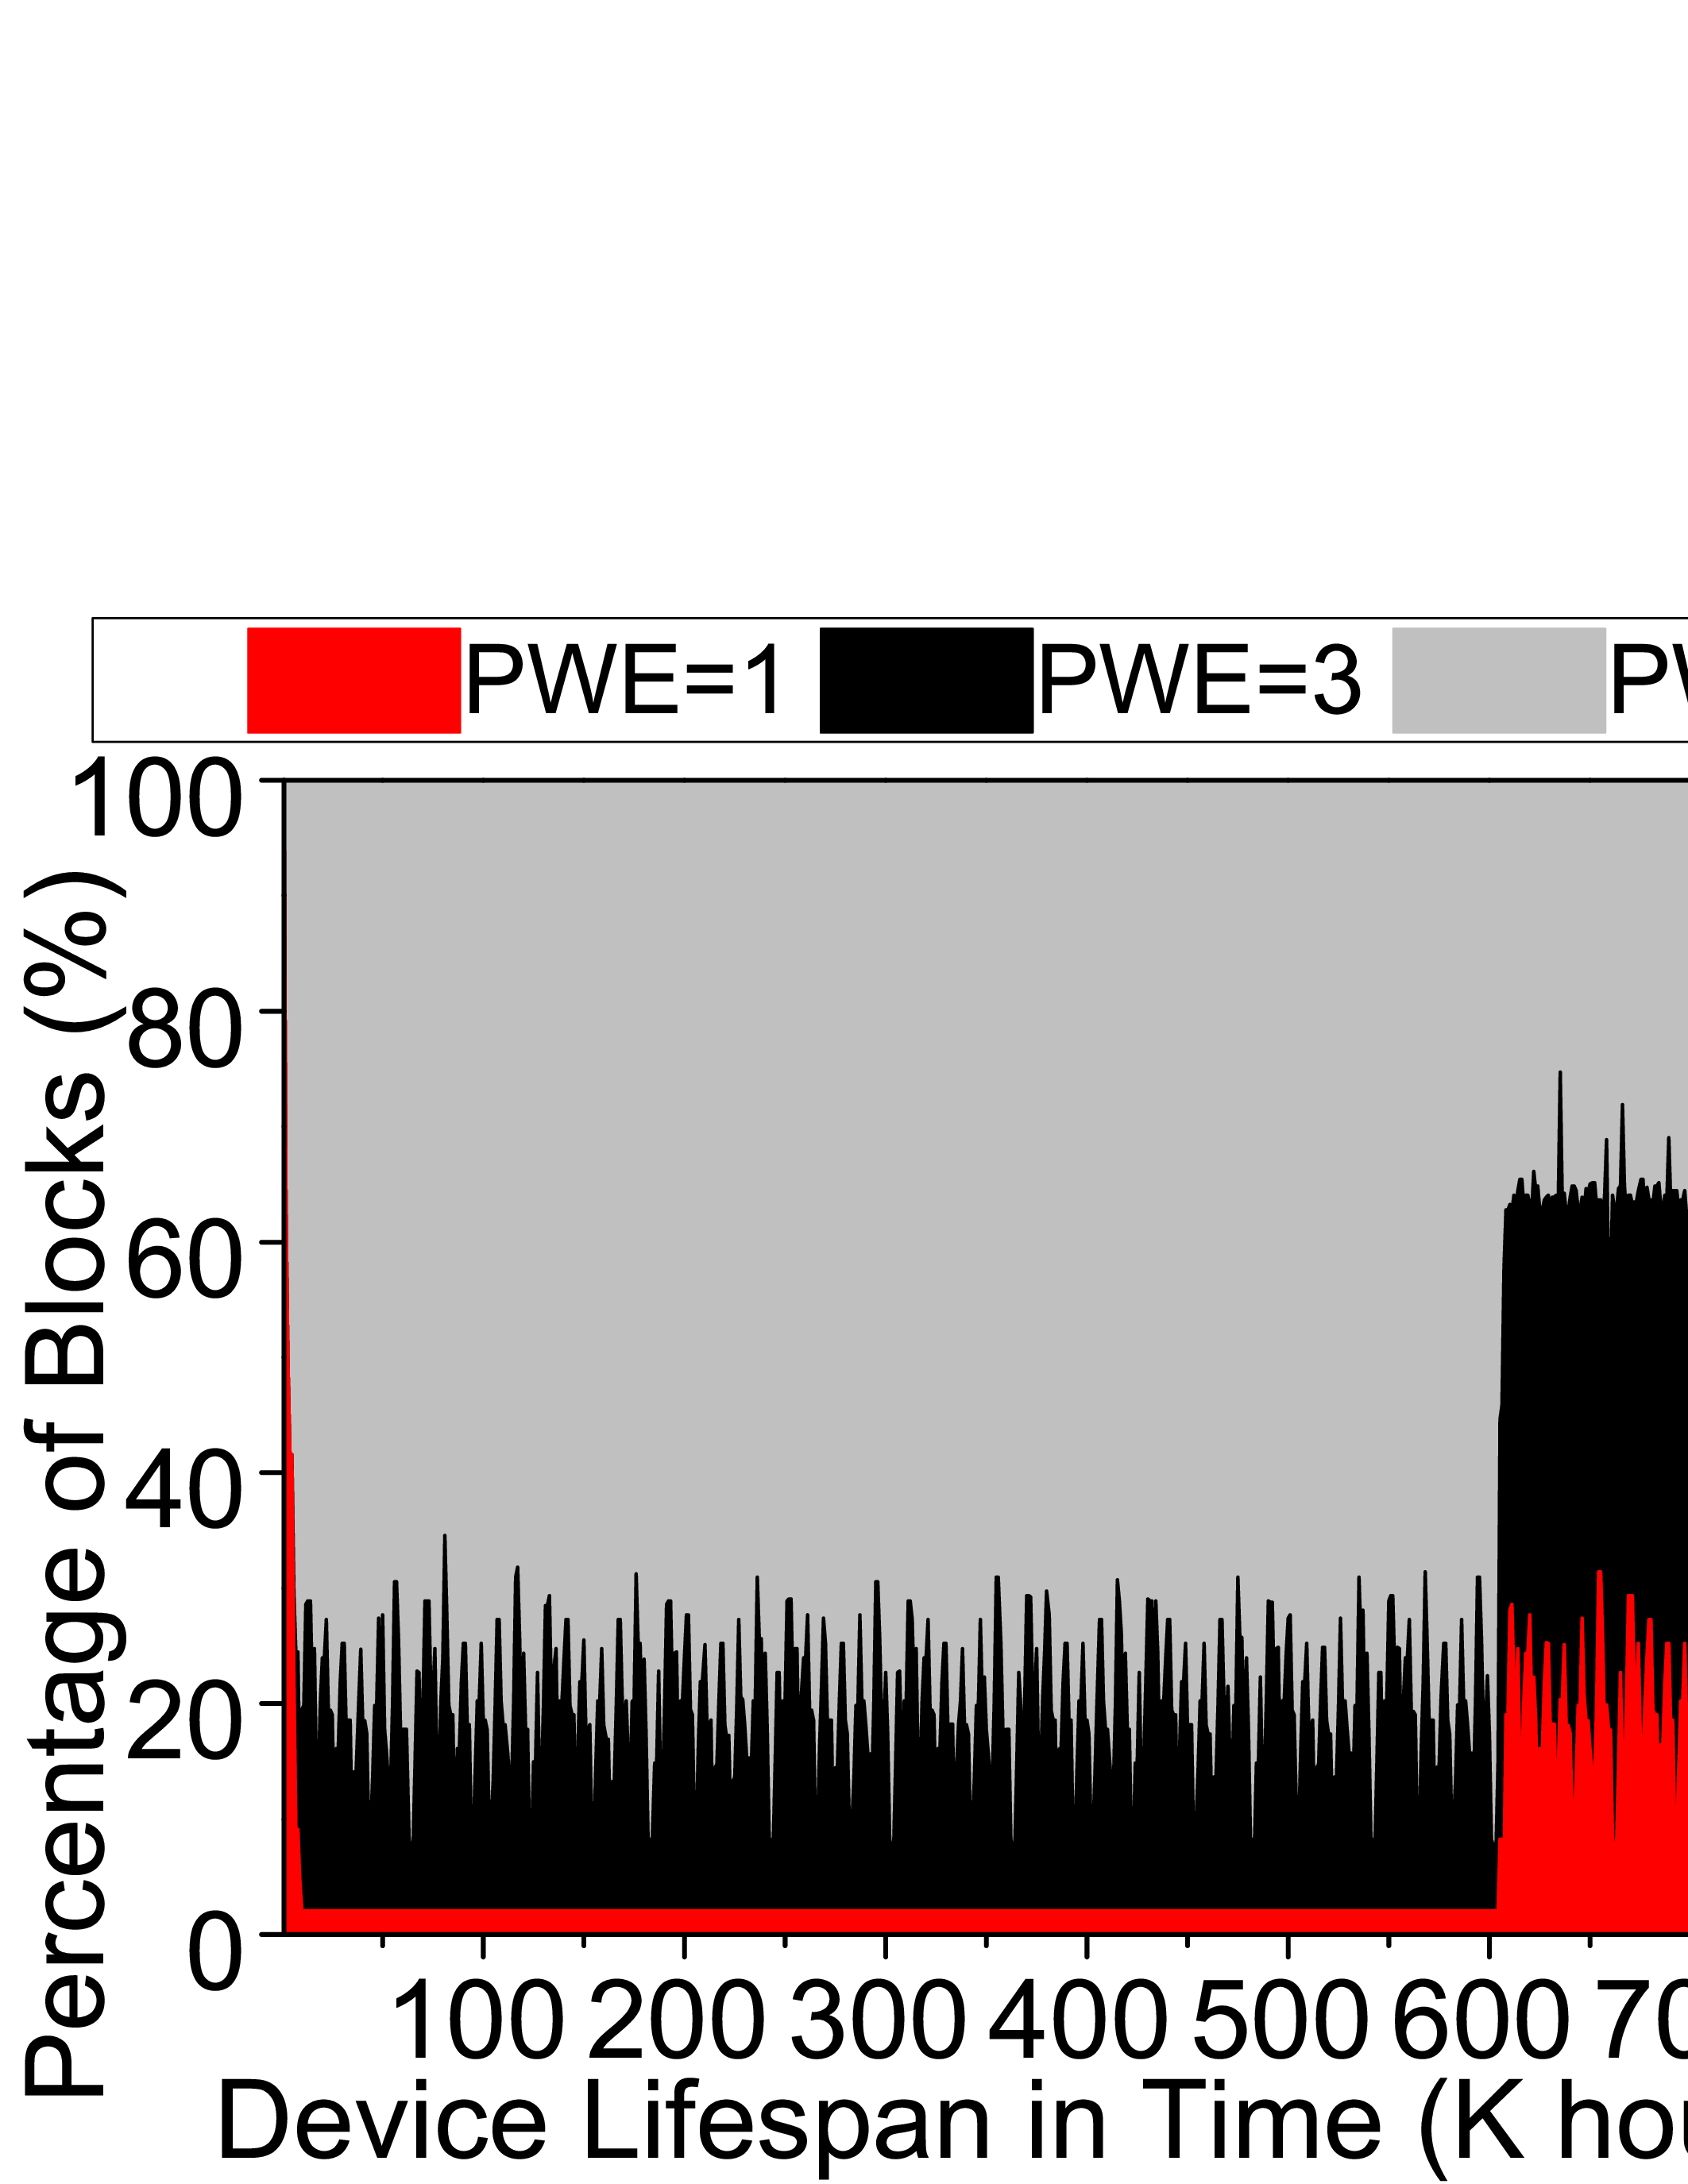}
		\caption{wdev\textunderscore2 in Normal}\label{fig:pwe-sense-drift-wdev_2-normal}
	\end{subfigure}
	\begin{subfigure}{.33\linewidth}
		\centering
		\includegraphics[width=0.99\linewidth]{graphs-app/pwe-wdev_2-strong.eps}
		\caption{wdev\textunderscore2 in Strong}\label{fig:pwe-sense-drift-wdev_2-strong}
	\end{subfigure}
\caption{Percentages of blocks with 2, 4, and 8 states, when running \emph{wdev\textunderscore2} on Weak, Normal, and Strong devices.}
\label{fig:pwe-sense-drift-wdev_2}
\end{figure*}

\begin{figure*}
\centering
	\begin{subfigure}{.33\linewidth}
		\centering
		\includegraphics[width=0.99\linewidth]{graphs-app/pwe-rsrch_0-weak.eps}
		\caption{rsrch\textunderscore0 in Weak}\label{fig:pwe-sense-drift-rsrch_0-weak}
	\end{subfigure}
	\begin{subfigure}{.33\linewidth}
		\centering
		\includegraphics[width=0.99\linewidth]{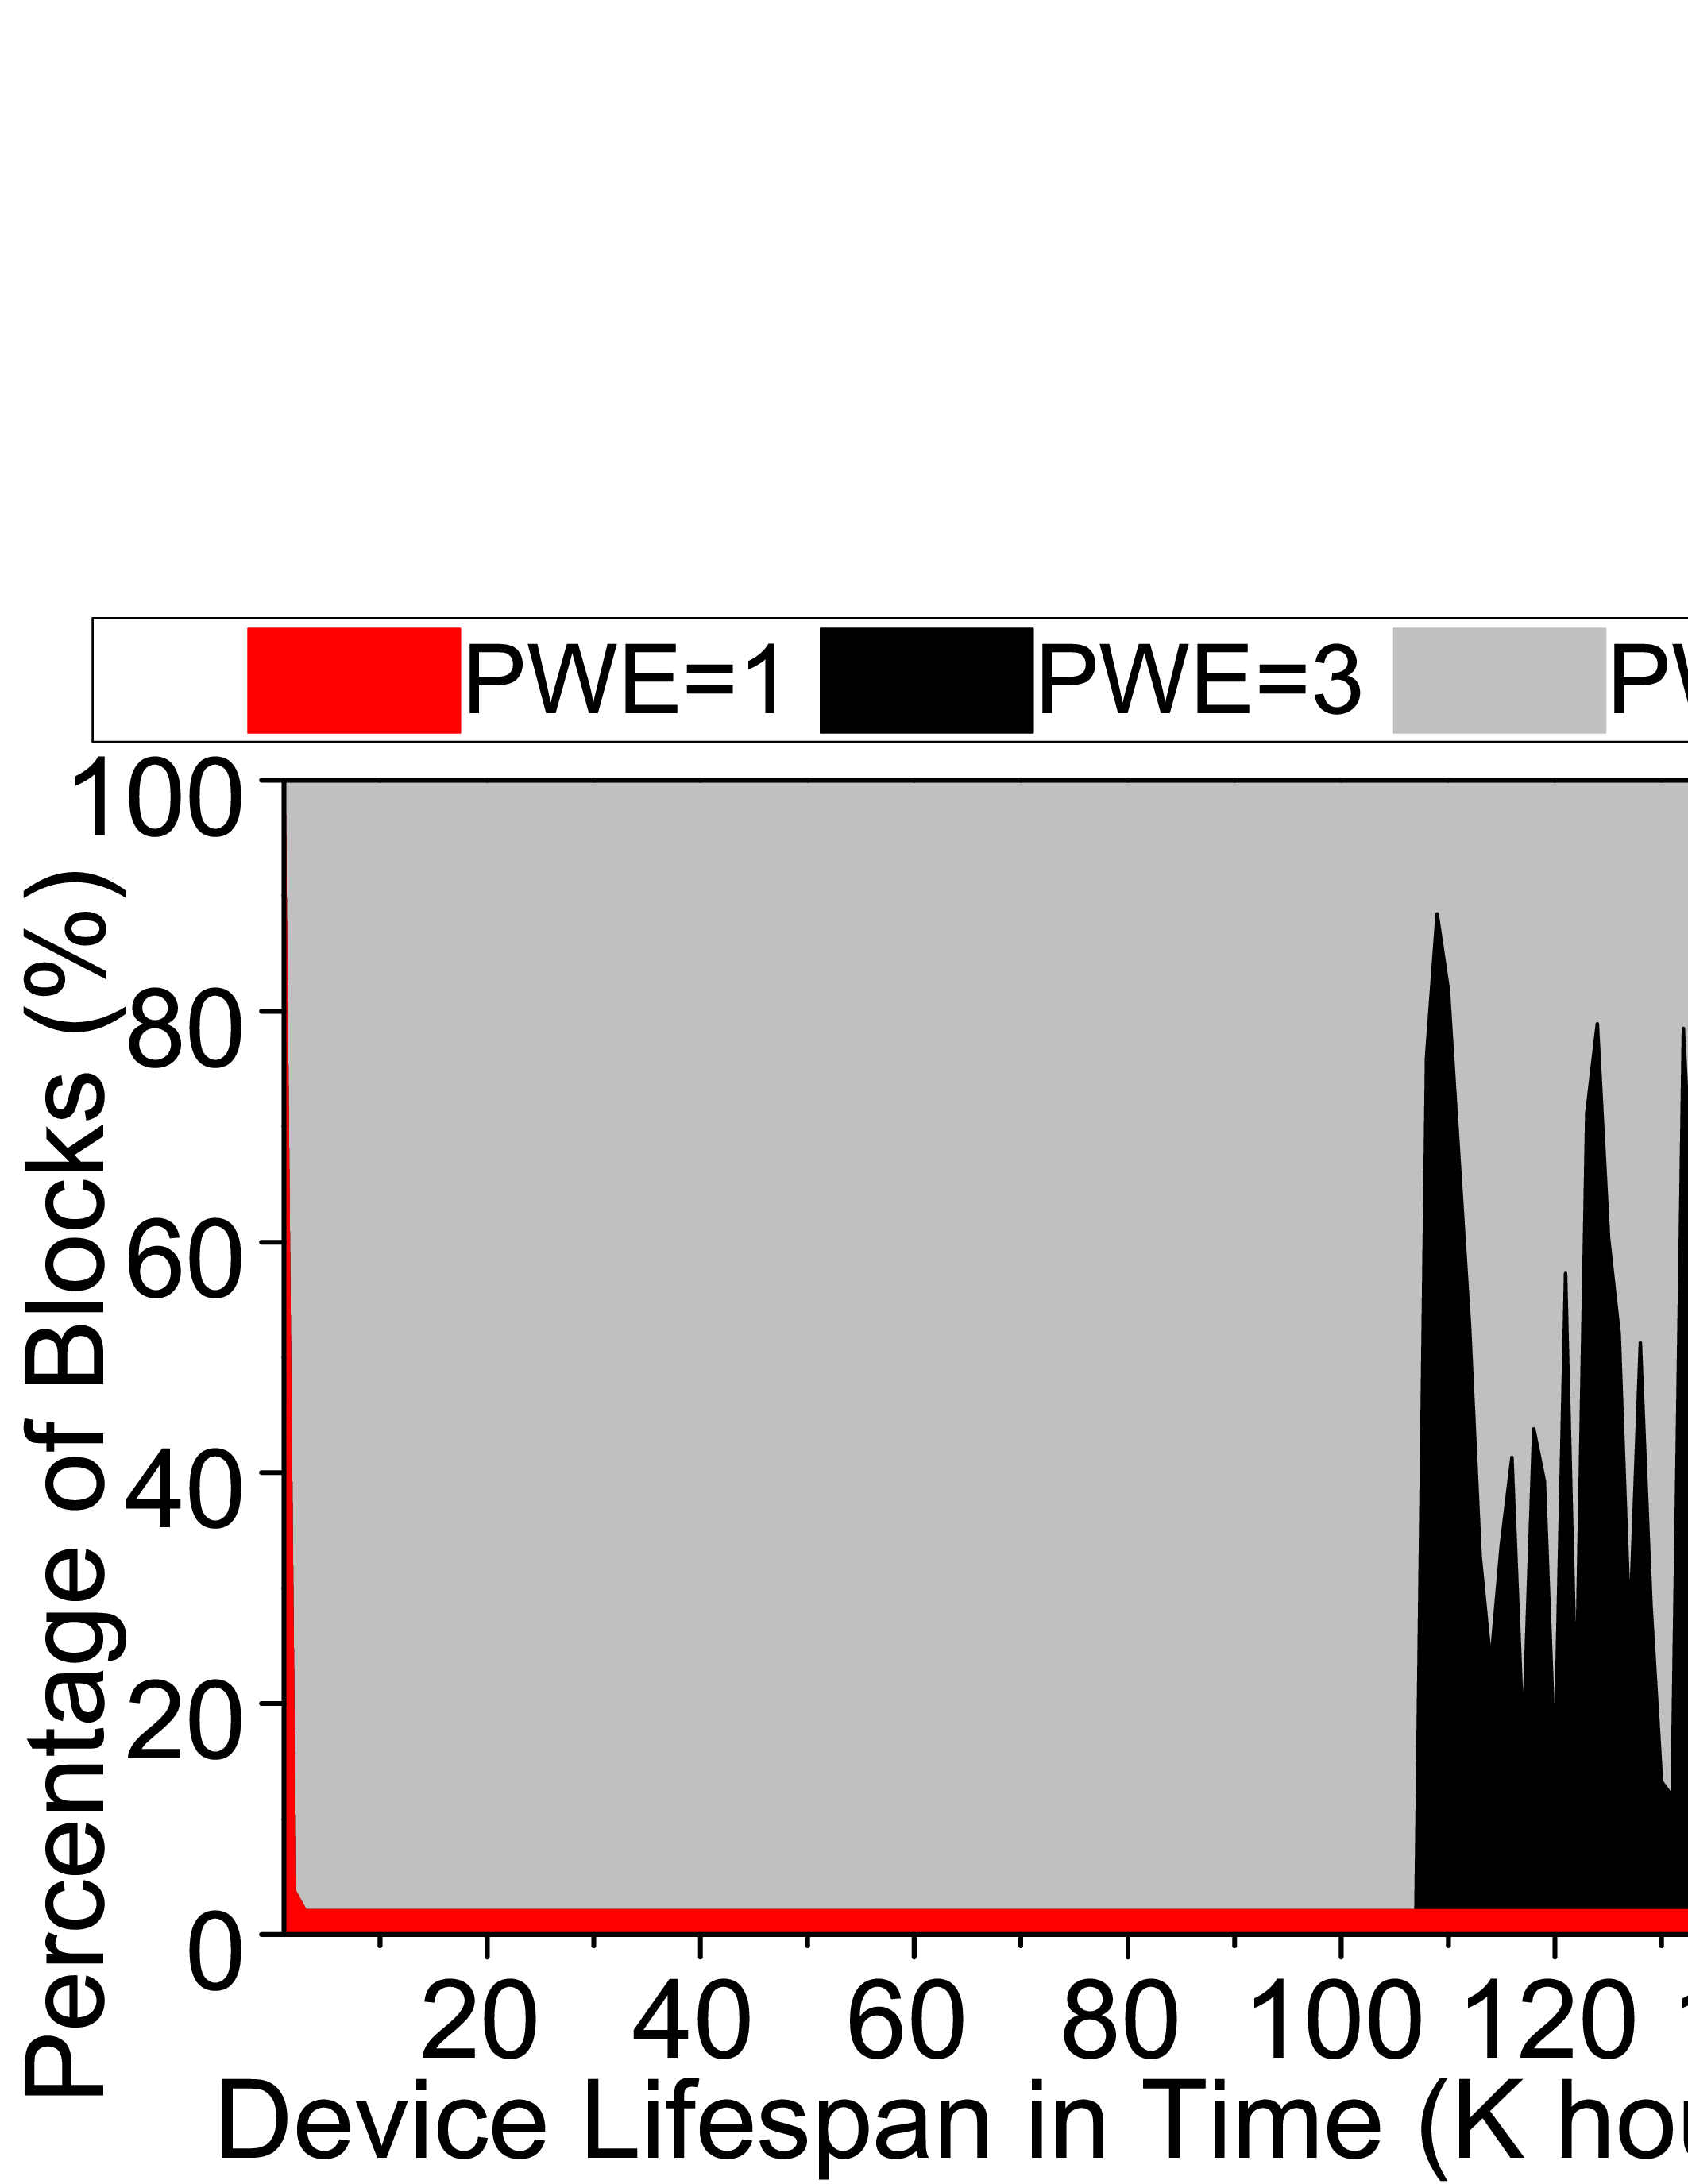}
		\caption{rsrch\textunderscore0 in Normal}\label{fig:pwe-sense-drift-rsrch_0-normal}
	\end{subfigure}
	\begin{subfigure}{.33\linewidth}
		\centering
		\includegraphics[width=0.99\linewidth]{graphs-app/pwe-rsrch_0-strong.eps}
		\caption{rsrch\textunderscore0 in Strong}\label{fig:pwe-sense-drift-rsrch_0-strong}
	\end{subfigure}
\caption{Percentages of blocks with 2, 4, and 8 states, when running \emph{rsrch\textunderscore0} on Weak, Normal, and Strong devices.}
\label{fig:pwe-sense-drift-rsrch_0}
\end{figure*}

\clearpage
\section{Sensitivity Tests: Varying Support Mode Counts (2, 3, 4, and 5-Mode)}

\begin{figure*}
\centering
	\begin{subfigure}{.24\linewidth}
		\centering
		\includegraphics[width=0.99\linewidth]{graphs-app/pwe-hm_0-m2.eps}
		\caption{hm\textunderscore0 in 2-Mode}\label{fig:pwe-sense-mode-hm_0-m2}
	\end{subfigure}
	\begin{subfigure}{.24\linewidth}
		\centering
		\includegraphics[width=0.99\linewidth]{graphs/pwe-hm_0.eps}
		\caption{hm\textunderscore0 in 3-Mode}\label{fig:pwe-sense-mode-hm_0-m3}
	\end{subfigure}
	\begin{subfigure}{.24\linewidth}
		\centering
		\includegraphics[width=0.99\linewidth]{graphs-app/pwe-hm_0-m4.eps}
		\caption{hm\textunderscore0 in 4-Model}\label{fig:pwe-sense-mode-hm_0-m4}
	\end{subfigure}
	\begin{subfigure}{.24\linewidth}
		\centering
		\includegraphics[width=0.99\linewidth]{graphs-app/pwe-hm_0-m5.eps}
		\caption{hm\textunderscore0 in 5-Model}\label{fig:pwe-sense-mode-hm_0-m5}
	\end{subfigure}
\caption{Percentages of blocks with different states, when running \emph{hm\textunderscore0} in 2-Mode, 3-Mode, 4-Mode, and 5-Mode devices.}
\label{fig:pwe-sense-mode-hm_0}
%\vspace{-6pt}
\end{figure*}

\begin{figure*}
\centering
	\begin{subfigure}{.24\linewidth}
		\centering
		\includegraphics[width=0.99\linewidth]{graphs-app/pwe-prn_0-m2.eps}
		\caption{prn\textunderscore0 in 2-Mode}\label{fig:pwe-sense-mode-prn_0-m2}
	\end{subfigure}
	\begin{subfigure}{.24\linewidth}
		\centering
		\includegraphics[width=0.99\linewidth]{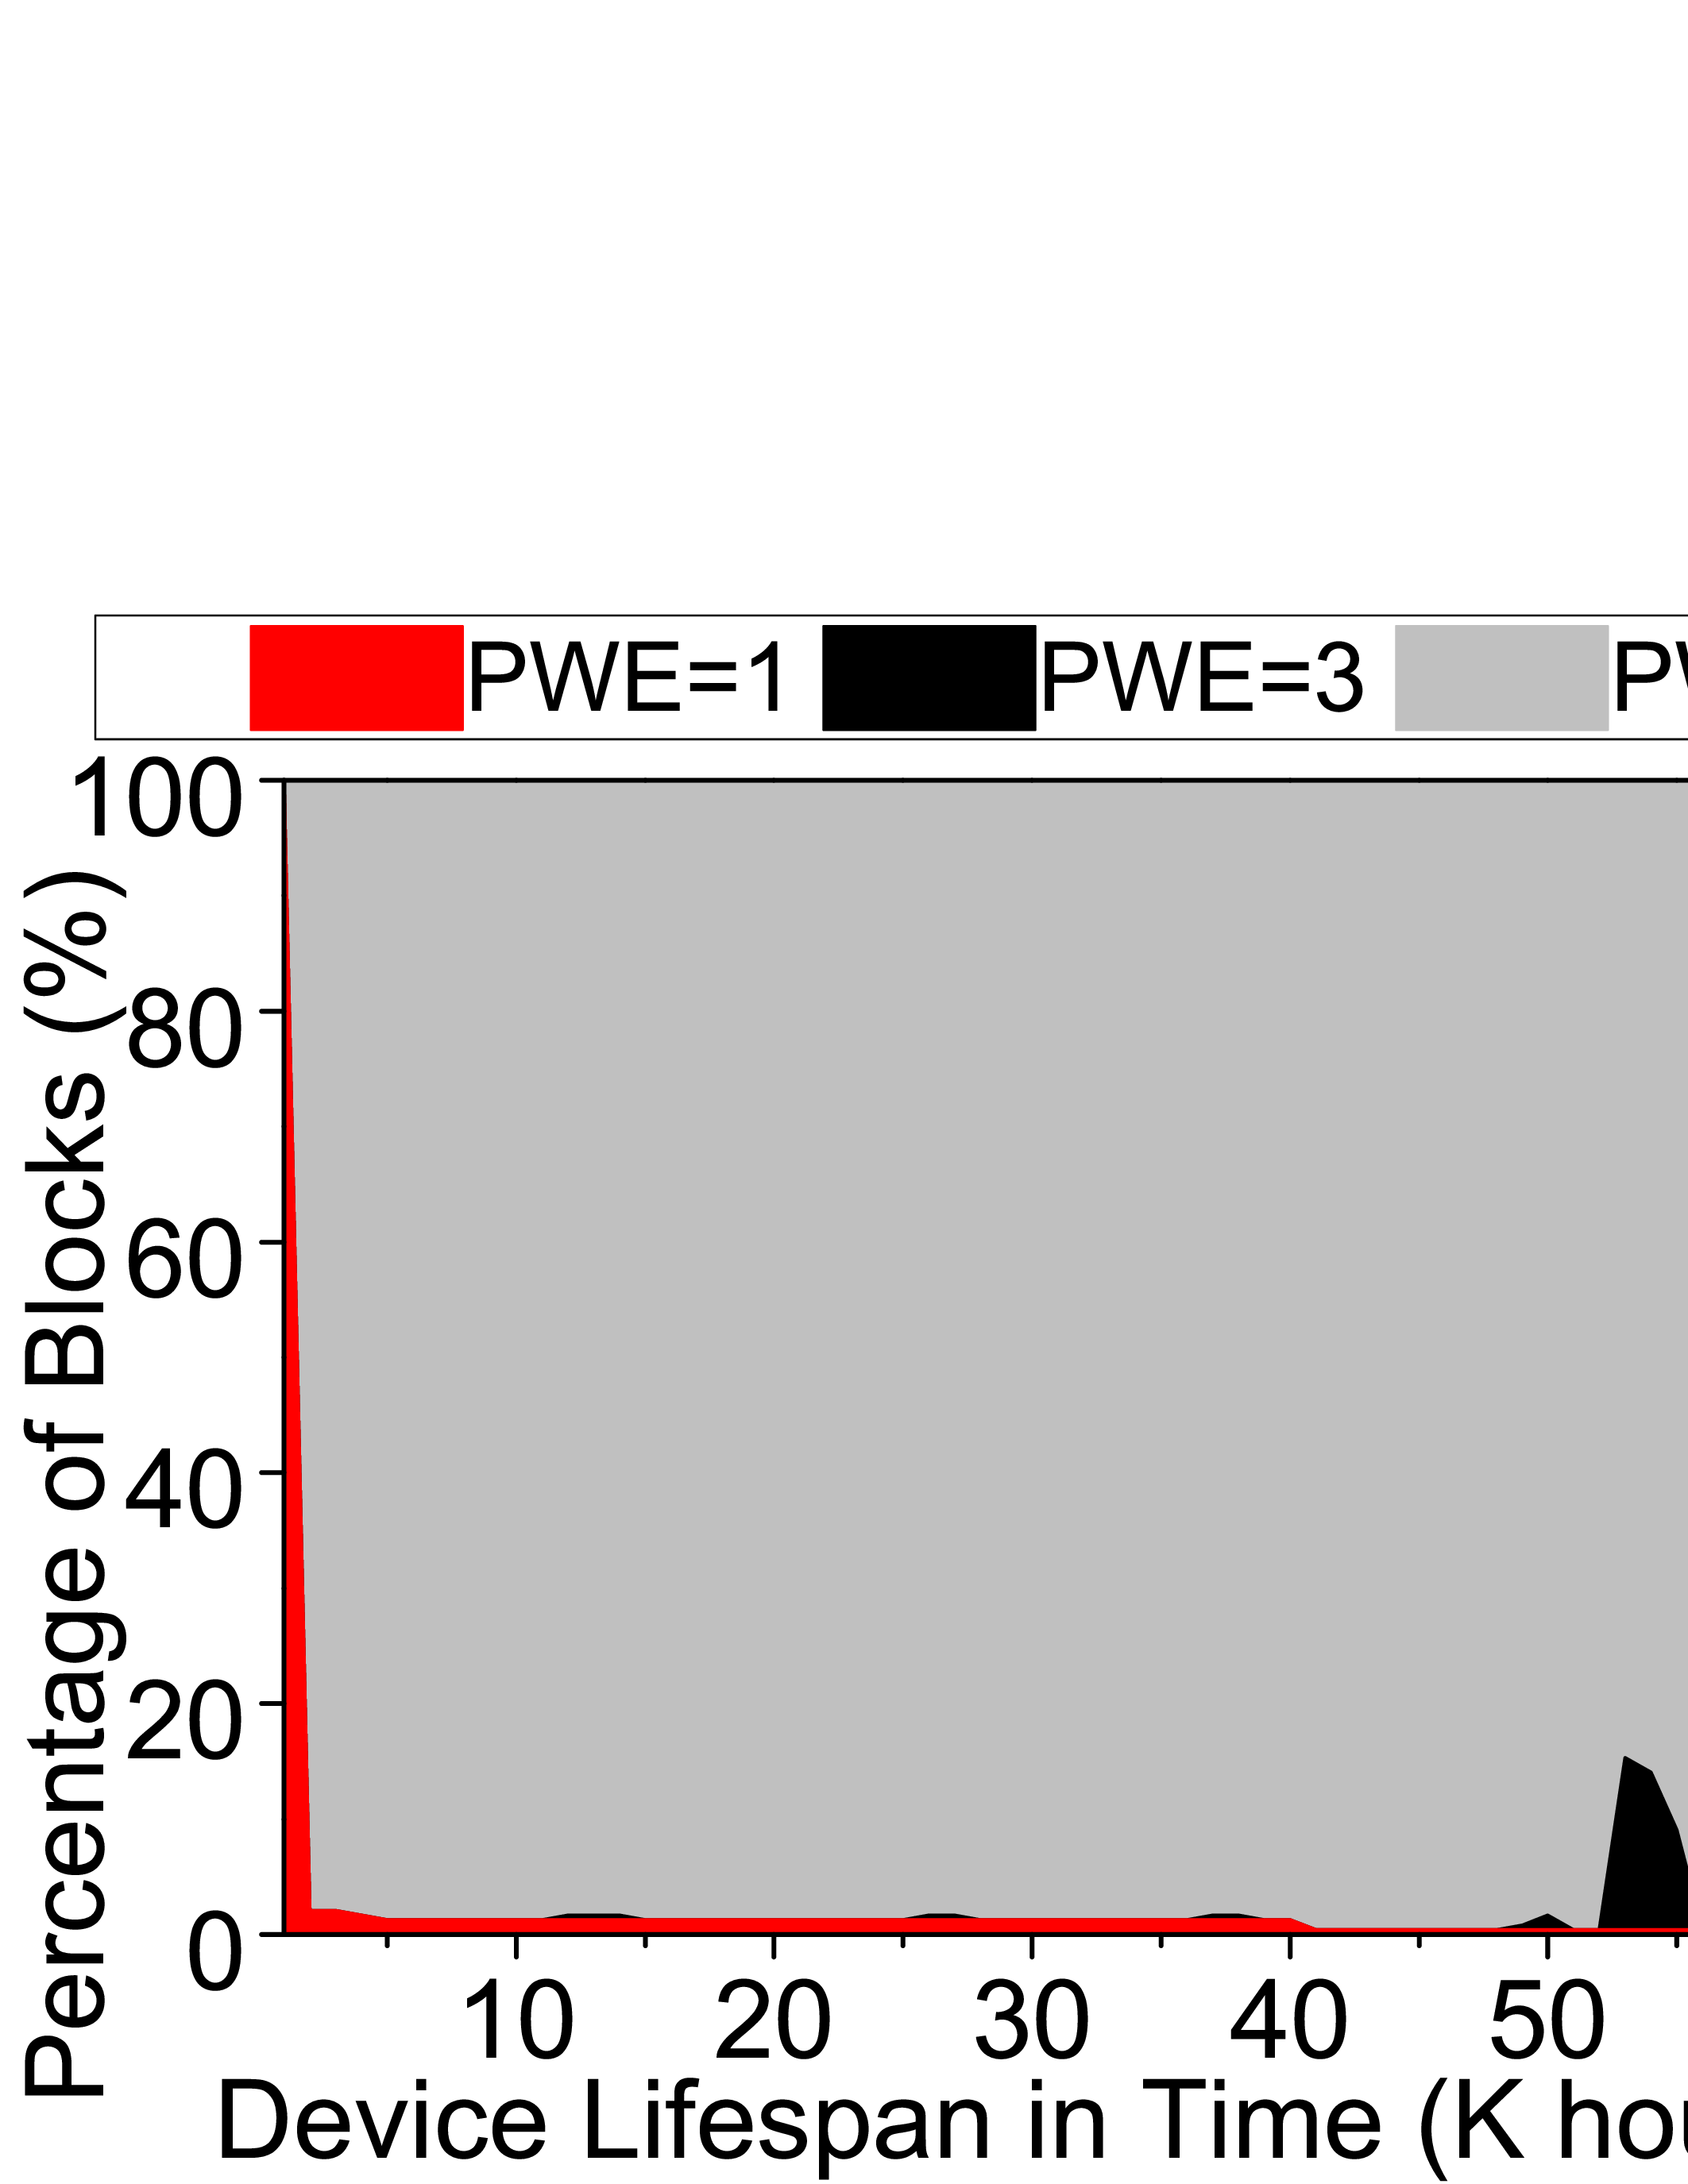}
		\caption{prn\textunderscore0 in 3-Mode}\label{fig:pwe-sense-mode-prn_0-m3}
	\end{subfigure}
	\begin{subfigure}{.24\linewidth}
		\centering
		\includegraphics[width=0.99\linewidth]{graphs-app/pwe-prn_0-m4.eps}
		\caption{prn\textunderscore0 in 4-Model}\label{fig:pwe-sense-mode-prn_0-m4}
	\end{subfigure}
	\begin{subfigure}{.24\linewidth}
		\centering
		\includegraphics[width=0.99\linewidth]{graphs-app/pwe-prn_0-m5.eps}
		\caption{prn\textunderscore0 in 5-Model}\label{fig:pwe-sense-mode-prn_0-m5}
	\end{subfigure}
\caption{Percentages of blocks with different states, when running \emph{prn\textunderscore0} in 2-Mode, 3-Mode, 4-Mode, and 5-Mode devices.}
\label{fig:pwe-sense-mode-prn_0}
%\vspace{-6pt}
\end{figure*}

\begin{figure*}
\centering
	\begin{subfigure}{.24\linewidth}
		\centering
		\includegraphics[width=0.99\linewidth]{graphs-app/pwe-prn_1-m2.eps}
		\caption{prn\textunderscore1 in 2-Mode}\label{fig:pwe-sense-mode-prn_1-m2}
	\end{subfigure}
	\begin{subfigure}{.24\linewidth}
		\centering
		\includegraphics[width=0.99\linewidth]{graphs/pwe-prn_1.eps}
		\caption{prn\textunderscore1 in 3-Mode}\label{fig:pwe-sense-mode-prn_1-m3}
	\end{subfigure}
	\begin{subfigure}{.24\linewidth}
		\centering
		\includegraphics[width=0.99\linewidth]{graphs-app/pwe-prn_1-m4.eps}
		\caption{prn\textunderscore1 in 4-Model}\label{fig:pwe-sense-mode-prn_1-m4}
	\end{subfigure}
	\begin{subfigure}{.24\linewidth}
		\centering
		\includegraphics[width=0.99\linewidth]{graphs-app/pwe-prn_1-m5.eps}
		\caption{prn\textunderscore1 in 5-Model}\label{fig:pwe-sense-mode-prn_1-m5}
	\end{subfigure}
\caption{Percentages of blocks with different states, when running \emph{prn\textunderscore1} in 2-Mode, 3-Mode, 4-Mode, and 5-Mode devices.}
\label{fig:pwe-sense-mode-prn_1}
%\vspace{-6pt}
\end{figure*}

\begin{figure*}
\centering
	\begin{subfigure}{.24\linewidth}
		\centering
		\includegraphics[width=0.99\linewidth]{graphs-app/pwe-proj_0-m2.eps}
		\caption{proj\textunderscore0 in 2-Mode}\label{fig:pwe-sense-mode-proj_0-m2}
	\end{subfigure}
	\begin{subfigure}{.24\linewidth}
		\centering
		\includegraphics[width=0.99\linewidth]{graphs/pwe-proj_0.eps}
		\caption{proj\textunderscore0 in 3-Mode}\label{fig:pwe-sense-mode-proj_0-m3}
	\end{subfigure}
	\begin{subfigure}{.24\linewidth}
		\centering
		\includegraphics[width=0.99\linewidth]{graphs-app/pwe-proj_0-m4.eps}
		\caption{proj\textunderscore0 in 4-Model}\label{fig:pwe-sense-mode-proj_0-m4}
	\end{subfigure}
	\begin{subfigure}{.24\linewidth}
		\centering
		\includegraphics[width=0.99\linewidth]{graphs-app/pwe-proj_0-m5.eps}
		\caption{proj\textunderscore0 in 5-Model}\label{fig:pwe-sense-mode-proj_0-m5}
	\end{subfigure}
\caption{Percentages of blocks with different states, when running \emph{proj\textunderscore0} in 2-Mode, 3-Mode, 4-Mode, and 5-Mode devices.}
\label{fig:pwe-sense-mode-proj_0}
%\vspace{-6pt}
\end{figure*}

\begin{figure*}
\centering
	\begin{subfigure}{.24\linewidth}
		\centering
		\includegraphics[width=0.99\linewidth]{graphs-app/pwe-prxy_0-m2.eps}
		\caption{prxy\textunderscore0 in 2-Mode}\label{fig:pwe-sense-mode-prxy_0-m2}
	\end{subfigure}
	\begin{subfigure}{.24\linewidth}
		\centering
		\includegraphics[width=0.99\linewidth]{graphs/pwe-prxy_0.eps}
		\caption{prxy\textunderscore0 in 3-Mode}\label{fig:pwe-sense-mode-prxy_0-m3}
	\end{subfigure}
	\begin{subfigure}{.24\linewidth}
		\centering
		\includegraphics[width=0.99\linewidth]{graphs-app/pwe-prxy_0-m4.eps}
		\caption{prxy\textunderscore0 in 4-Model}\label{fig:pwe-sense-mode-prxy_0-m4}
	\end{subfigure}
	\begin{subfigure}{.24\linewidth}
		\centering
		\includegraphics[width=0.99\linewidth]{graphs-app/pwe-prxy_0-m5.eps}
		\caption{prxy\textunderscore0 in 5-Model}\label{fig:pwe-sense-mode-prxy_0-m5}
	\end{subfigure}
\caption{Percentages of blocks with different states, when running \emph{prxy\textunderscore0} in 2-Mode, 3-Mode, 4-Mode, and 5-Mode devices.}
\label{fig:pwe-sense-mode-prxy_0}
%\vspace{-6pt}
\end{figure*}

\begin{figure*}
\centering
	\begin{subfigure}{.24\linewidth}
		\centering
		\includegraphics[width=0.99\linewidth]{graphs-app/pwe-mds_0-m2.eps}
		\caption{mds\textunderscore0 in 2-Mode}\label{fig:pwe-sense-mode-mds_0-m2}
	\end{subfigure}
	\begin{subfigure}{.24\linewidth}
		\centering
		\includegraphics[width=0.99\linewidth]{graphs/pwe-mds_0.eps}
		\caption{mds\textunderscore0 in 3-Mode}\label{fig:pwe-sense-mode-mds_0-m3}
	\end{subfigure}
	\begin{subfigure}{.24\linewidth}
		\centering
		\includegraphics[width=0.99\linewidth]{graphs-app/pwe-mds_0-m4.eps}
		\caption{mds\textunderscore0 in 4-Model}\label{fig:pwe-sense-mode-mds_0-m4}
	\end{subfigure}
	\begin{subfigure}{.24\linewidth}
		\centering
		\includegraphics[width=0.99\linewidth]{graphs-app/pwe-mds_0-m5.eps}
		\caption{mds\textunderscore0 in 5-Model}\label{fig:pwe-sense-mode-mds_0-m5}
	\end{subfigure}
\caption{Percentages of blocks with different states, when running \emph{mds\textunderscore0} in 2-Mode, 3-Mode, 4-Mode, and 5-Mode devices.}
\label{fig:pwe-sense-mode-mds_0}
%\vspace{-6pt}
\end{figure*}

\begin{figure*}
\centering
	\begin{subfigure}{.24\linewidth}
		\centering
		\includegraphics[width=0.99\linewidth]{graphs-app/pwe-src2_0-m2.eps}
		\caption{src2\textunderscore0 in 2-Mode}\label{fig:pwe-sense-mode-src2_0-m2}
	\end{subfigure}
	\begin{subfigure}{.24\linewidth}
		\centering
		\includegraphics[width=0.99\linewidth]{graphs/pwe-src2_0.eps}
		\caption{src2\textunderscore0 in 3-Mode}\label{fig:pwe-sense-mode-src2_0-m3}
	\end{subfigure}
	\begin{subfigure}{.24\linewidth}
		\centering
		\includegraphics[width=0.99\linewidth]{graphs-app/pwe-src2_0-m4.eps}
		\caption{src2\textunderscore0 in 4-Model}\label{fig:pwe-sense-mode-src2_0-m4}
	\end{subfigure}
	\begin{subfigure}{.24\linewidth}
		\centering
		\includegraphics[width=0.99\linewidth]{graphs-app/pwe-src2_0-m5.eps}
		\caption{src2\textunderscore0 in 5-Model}\label{fig:pwe-sense-mode-src2_0-m5}
	\end{subfigure}
\caption{Percentages of blocks with different states, when running \emph{src2\textunderscore0} in 2-Mode, 3-Mode, 4-Mode, and 5-Mode devices.}
\label{fig:pwe-sense-mode-src2_0}
%\vspace{-6pt}
\end{figure*}
